# Supplementary material for: Credit Scores: Performance and Equity
Source: arXiv:2409.00296 source file (2024-08-30)
Supplement: Supplementary file 2 [file appendix.tex]

\appendix
\counterwithin{figure}{section}
\counterwithin{table}{section}

\section{Additional Details and Analysis}\label{sec:appendixa}

\setcounter{figure}{0}
\setcounter{table}{0}

\subsection{Judgment Data}\label{appendixa1}

We obtained our Missouri judgment data from Paul Kiel and Annie  Waldman at ProPublica. The data they shared with us included all debt collection judgments in New Jersey, Missouri, and Cook County, Illinois, from 2008 to 2012.\footnote{The focus in their ProPublica article was Essex County, St. Louis City, St. Louis County, and Cook County due to the cities' high segregation indexes. Due to a peculiarity of the court system database, the Essex County window is slightly different: July 1, 2007, through June 30, 2012.}  Both Missouri and New Jersey have state-wide databases. The Missouri dataset was provided by Missouri's Office of the State Courts Administrator (OSCA) and included all debt collection cases filed in Associate Circuit Court for which OSCA has an electronic record through early 2014.\footnote{The max amount sought in associate circuit courts in Missouri is \$25,000.} For each case in Missouri, the data contained the following information: court (judicial circuit), county, case ID, filing Date, case type, disposition, plaintiff, plaintiff attorney, defendant, defendant date of birth, defendant address, defendant attorney, judgment amount, date of judgment satisfaction, date of first garnishment attempt.\footnote{The judgment amount was determined to be unreliable and is not used throughout this analysis.} Kiel and Waldman added two fields: a standard name for each plaintiff and a plaintiff type. Missouri's court system has some variation among the judicial circuits in how case types are categorized, so Keil and Waldman selected a range of case types that could be reasonably construed as debt collection cases in consultation with OSCA employees. For St. Louis City and County courts, these were: Breach of Contract, Promissory Note, Suit on Account, Contract /Account (Bulk), Misc Associate Civil-Other, Small Claims under \$100, Small Claims over \$100.\footnote{Together, the small claims and ``misc associate'' cases comprised less than four percent of cases.} They limited the dataset to cases that had resulted in a judgment.

We collapse this data to the zip code level.  As discussed in the Data Section of our paper, our main analysis focuses on Missouri, although we replicate our results with data from New Jersey and Illinois wherever feasible.  Within this data there are important differences in observable characteristics across majority black and non-majority black neighborhoods. Examples of such differences are documented in Figure \ref{fig:kde}. This figure shows kernel density estimates of various covariates used throughout this analysis.  Majority-black neighborhoods tend to have lower median credit scores, lower average incomes, lower house values, higher unemployment rates, and a higher share of divorced individuals. These differences cause concern that there could also be important differences in unobservable characteristics that vary with the racial composition of neighborhoods. We mitigate this concern by limiting our dataset to samples that only contain observations with common support over observables (\cite{crump2009dealing}). We use logistic regressions to restrict our dataset to a common support. More specifically, we estimate:

\begin{equation}
      \Phi(M_{ict}) = \beta_0 + \theta X_{ic}+\epsilon_{ic}
\end{equation}
where $M_{ict}$ is an indicator variable equal to one if observation $i$ in county $c$ in period $t$ is (or resides in) a majority black neighborhood and $X_{ict}$ is a vector of other controls for observation $i$ in county $c$ in period $t$.  Controls included quintiles of the credit score distributions, the fraction of IRS filings under \$25,000, between \$25,000-50,000, \$50,000-75,000, \$75,000-100,000, and over \$100,000, the average income, median credit scores, the Gini index of income inequality, 90+ days-past-due debt balances, unemployment and divorce rates, population density, median house value, and education attainment levels such as the fraction with at least a bachelors degree or with less than a high school diploma.

\subsection{Sensitivity Analysis}\label{appendixa2}

\subsubsection{Differences in Income and Credit Score}

In this section, we show how the coefficient on majority black changes as we add different controls to our neighborhood-level regression specification. 
 Column (1) of Table \ref{tab:creditworthiness} shows that majority-black neighborhoods have about 1.4 more judgments per every 100 people than non-black neighborhoods controlling only for county and year fixed effects. This coefficient implies that the baseline judgment rate in black neighborhoods is more than double that of non-majority black neighborhoods, where the average judgment rate is 1.26 judgments per 100 people. We progressively add additional control variables to our baseline specification to explore if and to what extent neighborhood-level income and credit score measures are driving the relationship between a neighborhood's racial composition and the number of judgments per 100 individuals. Column (2) of Table \ref{tab:creditworthiness} adds controls for average ZIP code level income and the fraction of IRS filings under \$25,000, between \$25,000-50,000, \$50,000-75,000, \$75,000-100,000, and over \$100,000, to the previous specification.  Column (3) in Table \ref{tab:creditworthiness} adds credit score quintiles and median credit score to the baseline specification. Column (4) adds income and credit score controls into the same specification. Column (5) adds controls for total delinquent debt balances, unemployment rate, median house value, the fraction of the population with a college education, the divorce rate, and population density. In this specification, we see that majority-black neighborhoods have a 56\% higher judgment rate than non-black neighborhoods. Column (6) uses a one-year lag of our income, credit score, and baseline controls, and the coefficient of interest changes only slightly.  

\subsubsection{Differences in Plaintiff Type}\label{appendixa22}

We explore if a specific plaintiff category drives differences in judgment rates across black and non-black zip codes.  For each zip code, we know the number of judgments awarded to the following plaintiff types:  auto, debt buyer, high-cost lender, major bank, medical, utility, and miscellaneous.  Debt buyers account for 48\% of plaintiffs in our sample.  Medical lenders, major banks, and high-cost lenders are the next largest plaintiff categories accounting for 20\%, 13\%, and 6\% of plaintiffs, respectively.  The other plaintiff categories are combined into the miscellaneous category.    

Our results are presented in Table \ref{tab:plaintiff_type}.  Each specification includes the income, credit score, and baseline controls discussed in Table \ref{tab:creditworthiness}, as well as county and year fixed effects. Column (1) repeats the main analysis and includes judgments from all plaintiff types (this is the same result presented in Column (5) of Table \ref{tab:creditworthiness}). Column (2) limits the outcome variable to only judgments obtained by debt buyers, Column (3) to major banks, Column (4) to medical companies, Column (5) to high-cost lenders, and Column (6) to any other lender.  

The coefficients estimated across each specification should not be directly compared due to differences in the baseline judgment rates in non-black neighborhoods across these different plaintiff types. For example, the judgment rate in non-black neighborhoods was 0.57 judgments per 100 people for debt buyers, 0.14 judgments per 100 people for miscellaneous lenders, and 0.08 judgments per 100 people for high-cost lenders. These baseline levels imply that majority-black neighborhoods have a 38\% higher judgment rate than non-black neighborhoods among debt buyers, 13\% higher among major banks, and a 156\% higher judgment rate among high-cost lenders. The racial gap in debt collection judgments is not prevalent among medical lenders. In our estimation, the miscellaneous lenders category consistently showed the highest racial imbalance in their lawsuits, followed closely by high-cost lenders.  

\subsubsection{Banks and Payday Lenders Neighborhood Analysis}

In this section, we explore differences in lending institutions across black and non-black neighborhoods at the zipcode-level.\footnote{The presence of payday lenders is likely the result of financial distress as opposed to the cause.  As such, we view these controls as an additional measure of the financial well-being of neighborhoods instead of a measure of credit access.} We use ArcGIS to create an index that measures the number of banks and payday lenders within five and 10-mile radii from each zip code's centroid.  We also use broadband access as a proxy for access to online credit markets and the share of credit reports unscored as a proxy for access to credit.\footnote{An unscored credit report is one in which there is not enough information on a consumer's credit report to issue a formal credit score.  This variable could serve as a measure of access to credit if unscored reports correlate with limited access to credit markets instead of a limited desire to obtain credit.}  We add these variables as controls to our main specification.  

This analysis only used data from 2008-2012, and thus our sample size is slightly smaller.  For context, we replicate the main results on this subsample of the data in Column (1) of Table \ref{tab:access_to_credit}.  Columns (2) and (3) add controls for broadband access and the share of unscored accounts in a zip code; both measures have no meaningful impact on our coefficient of interest.  Columns (4) and (5) add our controls for the number of banks and payday lenders within five and 10-mile radii.  We see that the number of banks negatively correlates with the judgment rate, while the number of payday lenders positively correlates with the number of judgments.  Adding these controls decreases the coefficient on the black majority by 14\%, though a large racial gap in the number of judgments issued across black and non-black communities remains.

\subsubsection{Alternative Credit Score and Other Additional Controls}

In Table \ref{tab:pp}, we replicate Table \ref{tab:creditworthiness} but add an alternative control for credit score calculated using a deep learning algorithm. The model consistently outperforms standard credit scoring models when predicting default rates (\cite{albanesi_vamossy}). This alternative credit score has more predictive power than the conventional credit score in predicting default. However, it does not mitigate the racial disparity we see in judgments across black and non-black communities. This finding supports that differences in credit scores, which measure a borrower's likelihood of default, are not the main factor driving the judgment gap between black and non-black communities.  

Each of our main specifications includes a static measure of housing values to control for differences in housing-related wealth across majority black and non-black neighborhoods. However, it is likely the case that neighborhoods experience differential housing market dynamics. To address concerns that our static neighborhood-level measures of housing values could miss such dynamic differences across majority black and majority non-black neighborhoods, we add Zillow's annual zip code level measure of home prices to our model. We also know that differential mortgage denial rates exist across white and black neighborhoods (\cite{bartlett2021consumer}). We, therefore, supplement our model with HMDA data documenting mortgage denial rates by zip code to see if such differences can explain the disparity in debt collection judgments across black and non-black neighborhoods. 

Table \ref{tab:access_to_housing} presents these results.  Column (1) shows our preferred results on the subsample of data for which HMDA data is available, and Column (3) shows our preferred specification on the subsample of data for which Zillow data is available. Columns (2) and (4) show how our coefficient of interest changes when HMDA and Zillow data are added to the empirical model. Adding these controls decreases the coefficient on majority-black by 30\%, though a large racial gap in the number of judgments issued across black and non-black communities remains.

\subsubsection{Alternative Dependent Variables and Weighting}

Throughout our main neighborhood-level analysis, we focus on the number of judgments per 100 individuals as our primary outcome variable of interest. The results from that analysis suggest there are more judgments per 100 people in majority-black neighborhoods than in majority non-black neighborhoods. In Column (1) of Table \ref{tab:judgment_alternative} we instead document the share of cases that resulted in a judgment. We see that majority-black neighborhoods are three percentage points more likely to have a case result in a judgment. A lower share of settled cases before trial is the primary driving force behind this difference. Because settling cases pre-trial often requires a large lump sum payment, this finding provides suggestive evidence that defendants from majority non-black neighborhoods can better mitigate negative shocks.\footnote{Since settling a case often requires a one-time lump sum payment, defendants who settle tend to have worse subsequent credit outcomes (Cheng et al. 2019). This finding suggests that a lower propensity to settle cases before a trial could help defendants from majority-black neighborhoods in the long run.}  

We further alter our outcome variable of interest by normalizing by the number of judgments per 100 people with tax filings under \$25,000 as opposed to normalizing by the total population. This specification presents an alternative way to address concerns that the risk set of individuals potentially exposed to debt collection judgments differs across black and non-black neighborhoods. The results are presented in Columns (2) of Table \ref{tab:judgment_alternative}.  Column (4) presents similar results but with the number of judgments normalized by 100 people with subprime or worse credit. While these coefficients can not be directly compared to our previous results due to differences in the sample averages of judgments per 100 people and judgments per 100 people with an increased likelihood of default, we still see positive and statistically significant coefficients on our black majority indicator variable.  

Column (6) of Table \ref{tab:judgment_alternative} presents results that winsorized our primary outcome variable at the 99th percentile to mitigate the impact of outliers. The positive and statistically significant coefficient suggests that outliers are not driving our main findings. Lastly, we explore the impact of not using population weighting. Our main neighborhood-level analysis uses population weighting since we are interested in the aggregate and representative gap. However, as shown in Table \ref{tab:summary_statistics}, black zip codes are more populated than non-black zip codes, meaning the judgment gap could be magnified by (or potentially solely driven by) the decision to population weight our regressions. As such, we also run equally weighted regressions. We consistently find coefficients that are of very similar signs, magnitudes, and statistical significance, as evidenced by Columns (3), (5), and (7) that replicate our previous three results.

\subsubsection{Neighborhood Racial Composition}\label{appendixa26}

In this section, we show that our results are robust to using the share of black residents in a neighborhood instead of a binary measure. Columns (1) and (2) of Table \ref{tab:race_proxies} present this result.  Column (1) shows a positive and statistically significant coefficient on the share of black residents within a zip code. This result suggests that a neighborhood with only black residents would have 1.5 more judgments per 100 people than a similar neighborhood with no black residents, more than double the baseline judgment rate in non-majority black neighborhoods. Column (2) shows our preferred specification from Table \ref{tab:creditworthiness}, which uses our binary measure for a black neighborhood for comparison. Tables \ref{tab:debt_composition_share_black} and \ref{tab:judgment_type_share_black} in the appendix replicate our main neighborhood-level results (Tables \ref{tab:debt_composition} and \ref{tab:judgment_type} in the main text) using the share of black residents instead of a binary measure. Results are statistically and economically similar to the results from our primary analysis.    

Since many creditors do not collect racial demographic information, the main analysis focuses on disparities across majority black and majority non-black neighborhoods. One could explore the racial composition of defendants within a neighborhood; however, since racial demographic information is often not collected by creditors, it is not available in the court data. 

We instead use a Bayesian Improved Surname Geocoding (BISG) to estimate the racial composition of the defendant pool (Elliott et al., 2009).\footnote{Consumer Finance Protection Bureau’s Office of Research (OR), the Division of Supervision, Enforcement, and Fair Lending (SEFL) rely on a Bayesian Improved Surname Geocoding (BISG) proxy method.} This method combines publicly available geography- and surname-based information into a single proxy probability for an individual's race using the Bayes updating rule. This method involves constructing a probability of assignment to race based on demographic information associated with surname and then updating this probability using the demographic characteristics of the zip code associated with place of residence. The updating is performed through a Bayesian algorithm, which yields an integrated probability that can be used to proxy for an individual’s race and ethnicity. We again classify the defendant pool as majority-black if at least 50\% of the defendants in the debt collection data were predicted to be black. Information on the racial and ethnic composition of the U.S. population by geography comes from the Summary File 1 (SF1) from the 2010 Census, which provides counts of enumerated individuals by age, race, and ethnicity for various geographic area definitions including zip code tabulation areas.\footnote{Census blocks are the highest level of disaggregation (the smallest geography).} Research has found that this approach produces proxies that correlate highly with self-reported race and national origin and is more accurate than relying only on demographic information associated with a borrower’s last name or place of residence alone (CFBP Report, 2014).   

Vectors of six racial/ethnic probabilities for each listed surname (corrected for suppression and low-frequency surnames) are used as the first input into the BISG algorithm. This information calculates a prior probability of an individual's race/ethnicity. The algorithm updates these prior probabilities with geocoded ZCTA proportions for these groups from the 2010 Census SF1 files to generate posterior probabilities. Let J equal the number of names on the enhanced surname list plus one to account for names, not on the list and let K equal the number of ZCTA in the 2010 census with any population. We define the prior probability of a person’s race based on surname so that for a person with surname j = 1, ..., J on the list, the prior probability for the race, i = 1,...,6, is p(i|j) = proportion of all people with surname j who report being of the race i in the enhanced surname file (the probability of a selected race given surname). This probability is updated based on ZCTA residence. For ZCTA k = 1,...,K, r(k|i) = proportion of all people in redistributed SF1 file who self report being race i who reside in ZCTA k (the probability of a selected ZCTA of residence given race/ethnicity).  Let $u(i, j, k) = p(i|j) * r(k|i)$.  According to Bayes' Theorem and the assumption that the probability of residing in a given ZCTA given a person's race does not vary by surname, the updated (posterior) probability of being of race/ethnicity i given surname j and ZCTA of residence k can be calculated as follows:

\begin{equation}
 q(i|j,k)=\frac{u(i,j,k)}{u(1,j,k)+u(2,j,k)+u(3,j,k)+u(4,j,k)+u(5,j,k)+u(6,j,k)}  
\end{equation}

\noindent
Note that all parameters needed for BISG posterior probabilities are derived only from Census 2010 data and none from administrative sources.  
Columns (3)-(4) of Table A9 present the results. Once again, the results are positive and statistically significant.  We also replicate Table \ref{tab:debt_composition} using our BISG estimate of the racial composition of the defendant pool in Table \ref{tab:debt_composition_bisg}.  We find results that are similar in size and statistical significance.

\subsubsection{Selection on Unobservables}

We also investigated the impact of selection on unobservables on coefficient stability (\cite{oster_unobservable}). In particular, we used Column (5) of Table \ref{tab:creditworthiness} as our benchmark and found that given a selection on unobservables that is half the size of the selection on observables, our coefficient on majority-black is reduced to 0.53 with a 95\% confidence interval ranging from [0.26 to 0.81].\footnote{We bootstrapped our treatment coefficient estimates 100 times and assumed a maximum $R^2$ value of 0.9.}  This suggests that majority-black neighborhoods experience approximately 40\% more judgments than non-majority black neighborhoods.\footnote{We also examined the proportion of selection of unobservables to observables that would explain away our treatment effect. We found that a ratio of 1.91 with a 95\% confidence interval ranging from [0.89, 2.92] is sufficient to explain away our findings.}  This finding suggests that a racial gap is unlikely to be zero, even after controlling for unobservable characteristics.

\subsubsection{Additional Judgment Data Sources}

Lastly, we replicate our main results with zip code data from New Jersey and Cook County, Illinois. The results are presented in Table \ref{tab:summary_statistics_il_nj} and \ref{tab:debt_composition_nj_il}, which replicate Tables \ref{tab:summary_statistics} and \ref{tab:debt_composition} using data from New Jersey and Cook County, Illinois.\footnote{We cannot replicate Table \ref{tab:judgment_type} with this data as this information is not available for this sample.}  Table \ref{tab:summary_statistics_il_nj} shows that judgments per 100 people are larger in majority-black neighborhoods compared to majority non-black neighborhoods, while median income and median credit score tend to be lower. Table \ref{tab:debt_composition_nj_il} shows that credit scores, income levels, and debt characteristics are not driving the racial disparity in debt collection judgments. These results suggest that judgments are 18\% higher in black neighborhoods compared to non-black neighborhoods.  

We also relax the common support assumption and replicate our main results on the entire Missouri sample. These results are presented in tables \ref{tab:summary_statistics_off_common} through \ref{tab:judgment_type_off_common}.  Again, we find very similar results to our main specification, which uses only the common support sample, suggesting that omitted variables correlated with observable neighborhood characteristics are not biasing our results in any particular direction.

\subsubsection{Other Demographics}

In Table \ref{tab:race_other}, we replicate Table \ref{tab:creditworthiness} with additional controls for the share of the Hispanic and Asian population within each zip code. We do not observe any consistent judgment gap for Hispanic across our various specifications. However, we find that the share of the Asian population is negatively related to judgments. The share of black residents remains positive and statistically significant in each of the specifications.

\subsubsection{Non-linearities \& Higher Order Interactions}

Lastly, we investigate if causal machine learning techniques that allow for high-order interactions of observable characteristics can mitigate the disparity. This relies on the assumption that more information can be extracted from the interaction of multiple variables. More specifically, we adopt Double Machine Learning by \cite{chernozhukov2018double}, and implement Gradient Boosted Trees (GBT) and Random Forests in the first stages, with linear regression and robust standard errors in the second.\footnote{For more information about the GBT model, see \cite{friedman}.} Gradient Boosted Trees (GBT) is an ensemble learning approach that mitigates the tendency of tree-based models' to overfit training data. This is accomplished by recursively combining the forecasts of many over-simplified trees. The theory behind boosting proposes that a collection of weak learners as an ensemble create a single strong learner with improved stability over a single complex tree. 

At each step m, $1 \le m \le M$, of gradient boosting, an estimator, $h_m$, is computed on the residuals from the previous models' predictions. A critical part of the gradient boosting method is regularization by shrinkage as proposed by \cite{friedman}. This consists in modifying the update rule as follows:
\begin{equation}
    F_m(x) = F_{m-1}(x) + \nu \gamma_m h_m(x),
\end{equation}
where $h_m(x)$ represents a weak learner of fixed depth, $\gamma_m$ is the step length and $\nu$ is the learning rate or shrinkage factor.

The estimation procedure begins with fitting a shallow tree (e.g., with depth L = 1). Using the prediction residuals from the first tree, fit a second tree with the same shallow depth L. Weight the predictions of the second tree by $\nu \in (0,1)$ to prevent the model from overfitting the residuals, and then aggregate the forecasts of these two trees. At each step k, fit a shallow tree to the residuals from the model with k-1 trees, and add its prediction to the forecast of the ensemble with a shrinkage weight of $\nu$. Do this until a total of K trees is reached in the ensemble. For our GBT model, we split the data into three chunks: training set (60\%), holdout set (20\%), and testing set (20\%). We relied on XGBoost for the implementation of our GBT model (\cite{xgboost}).  We find that Double Machine Learning is unable to explain away the disparity. In particular, the estimates obtained in Table \ref{tab:dml} are similar to the ones obtained in Table \ref{tab:creditworthiness}.

\clearpage

\subsection*{Appendix Figures}\label{sec:fig}
\addcontentsline{toc}{section}{Figures}

\begin{figure}[!h]
\footnotesize
\begin{center}
\begin{subfigure}[b]{0.7\textwidth}
\includegraphics[width=\textwidth]{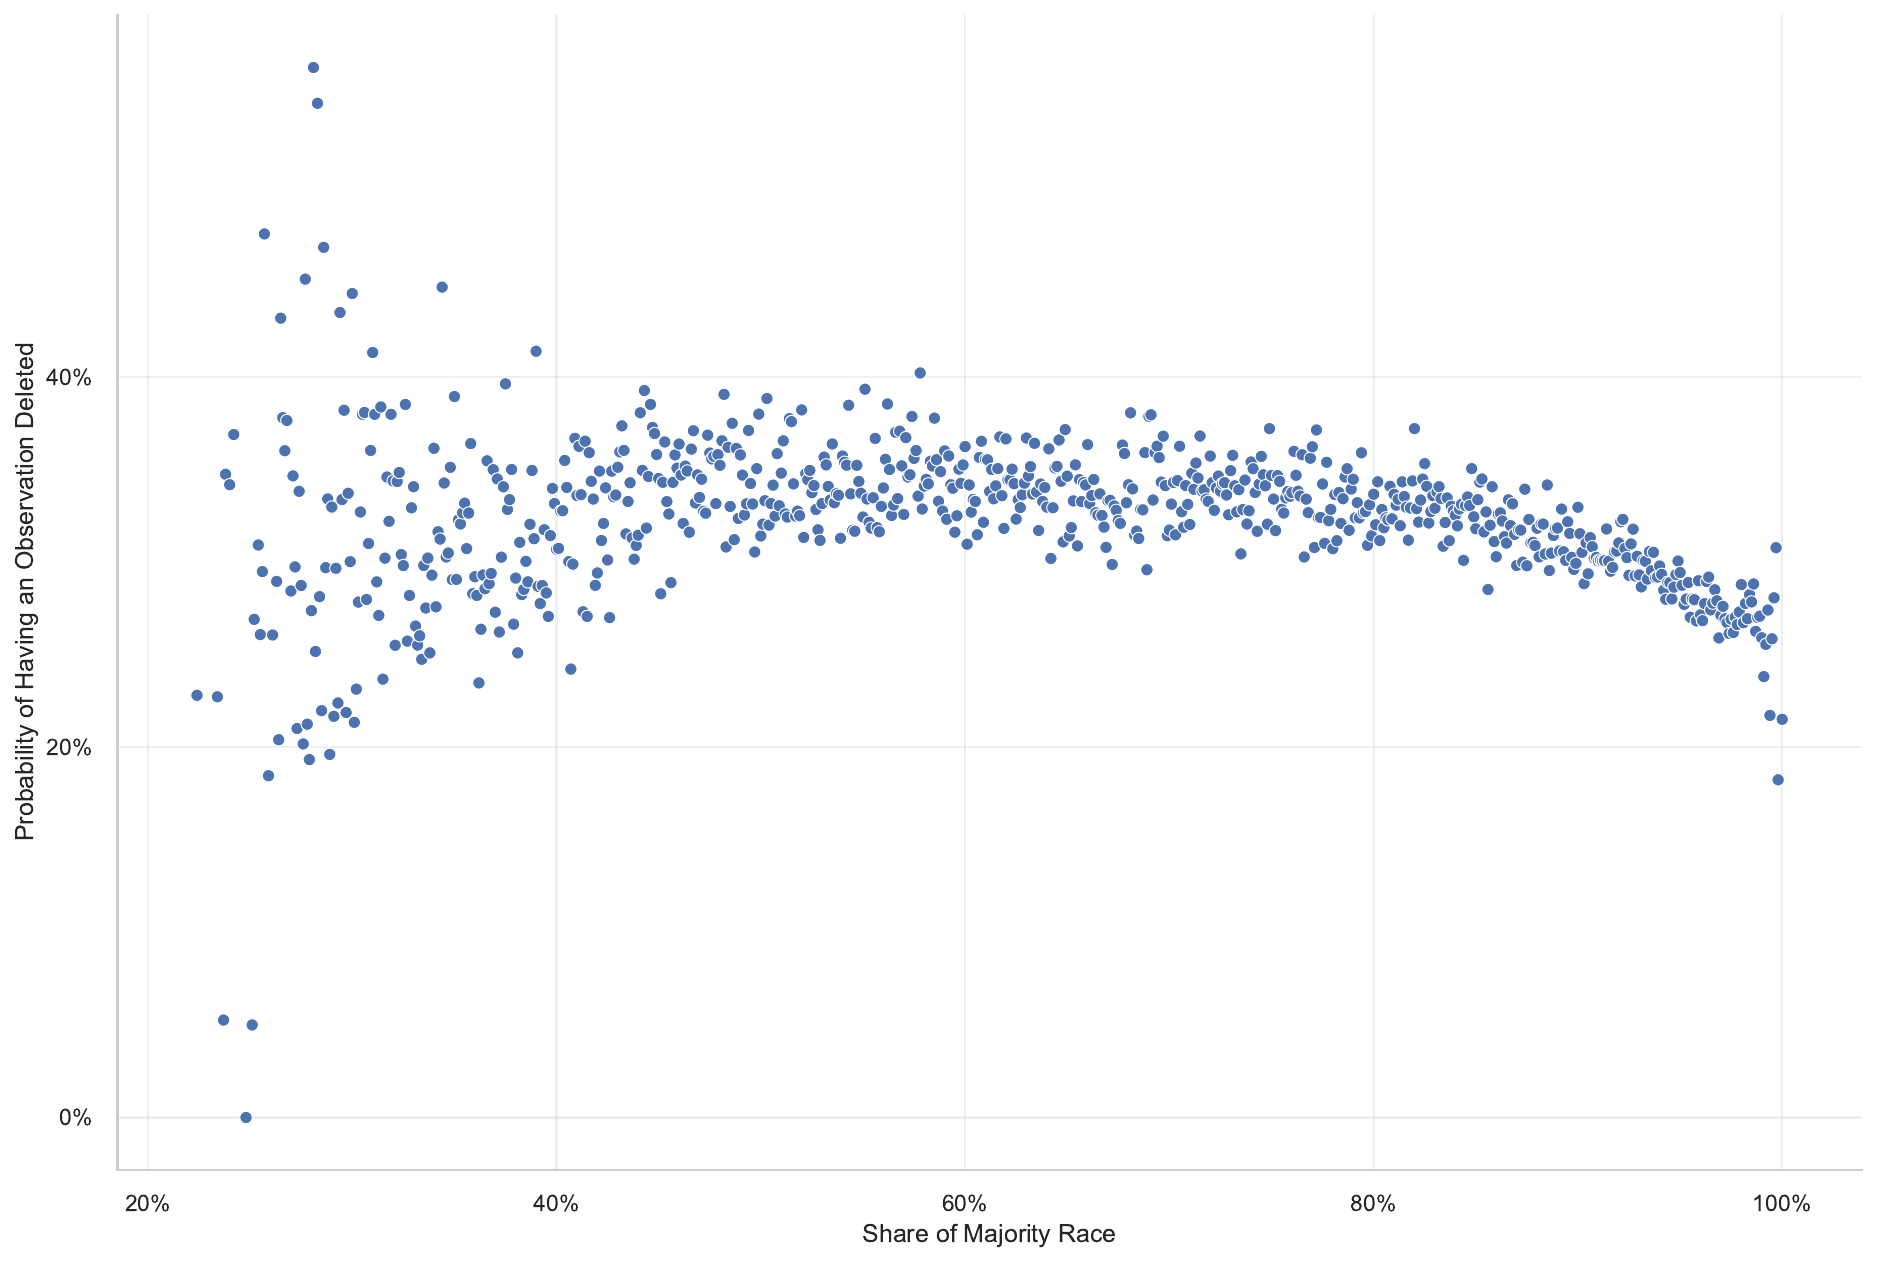}
\caption{}
\end{subfigure}
\begin{subfigure}[b]{0.7\textwidth}
\includegraphics[width=\textwidth]{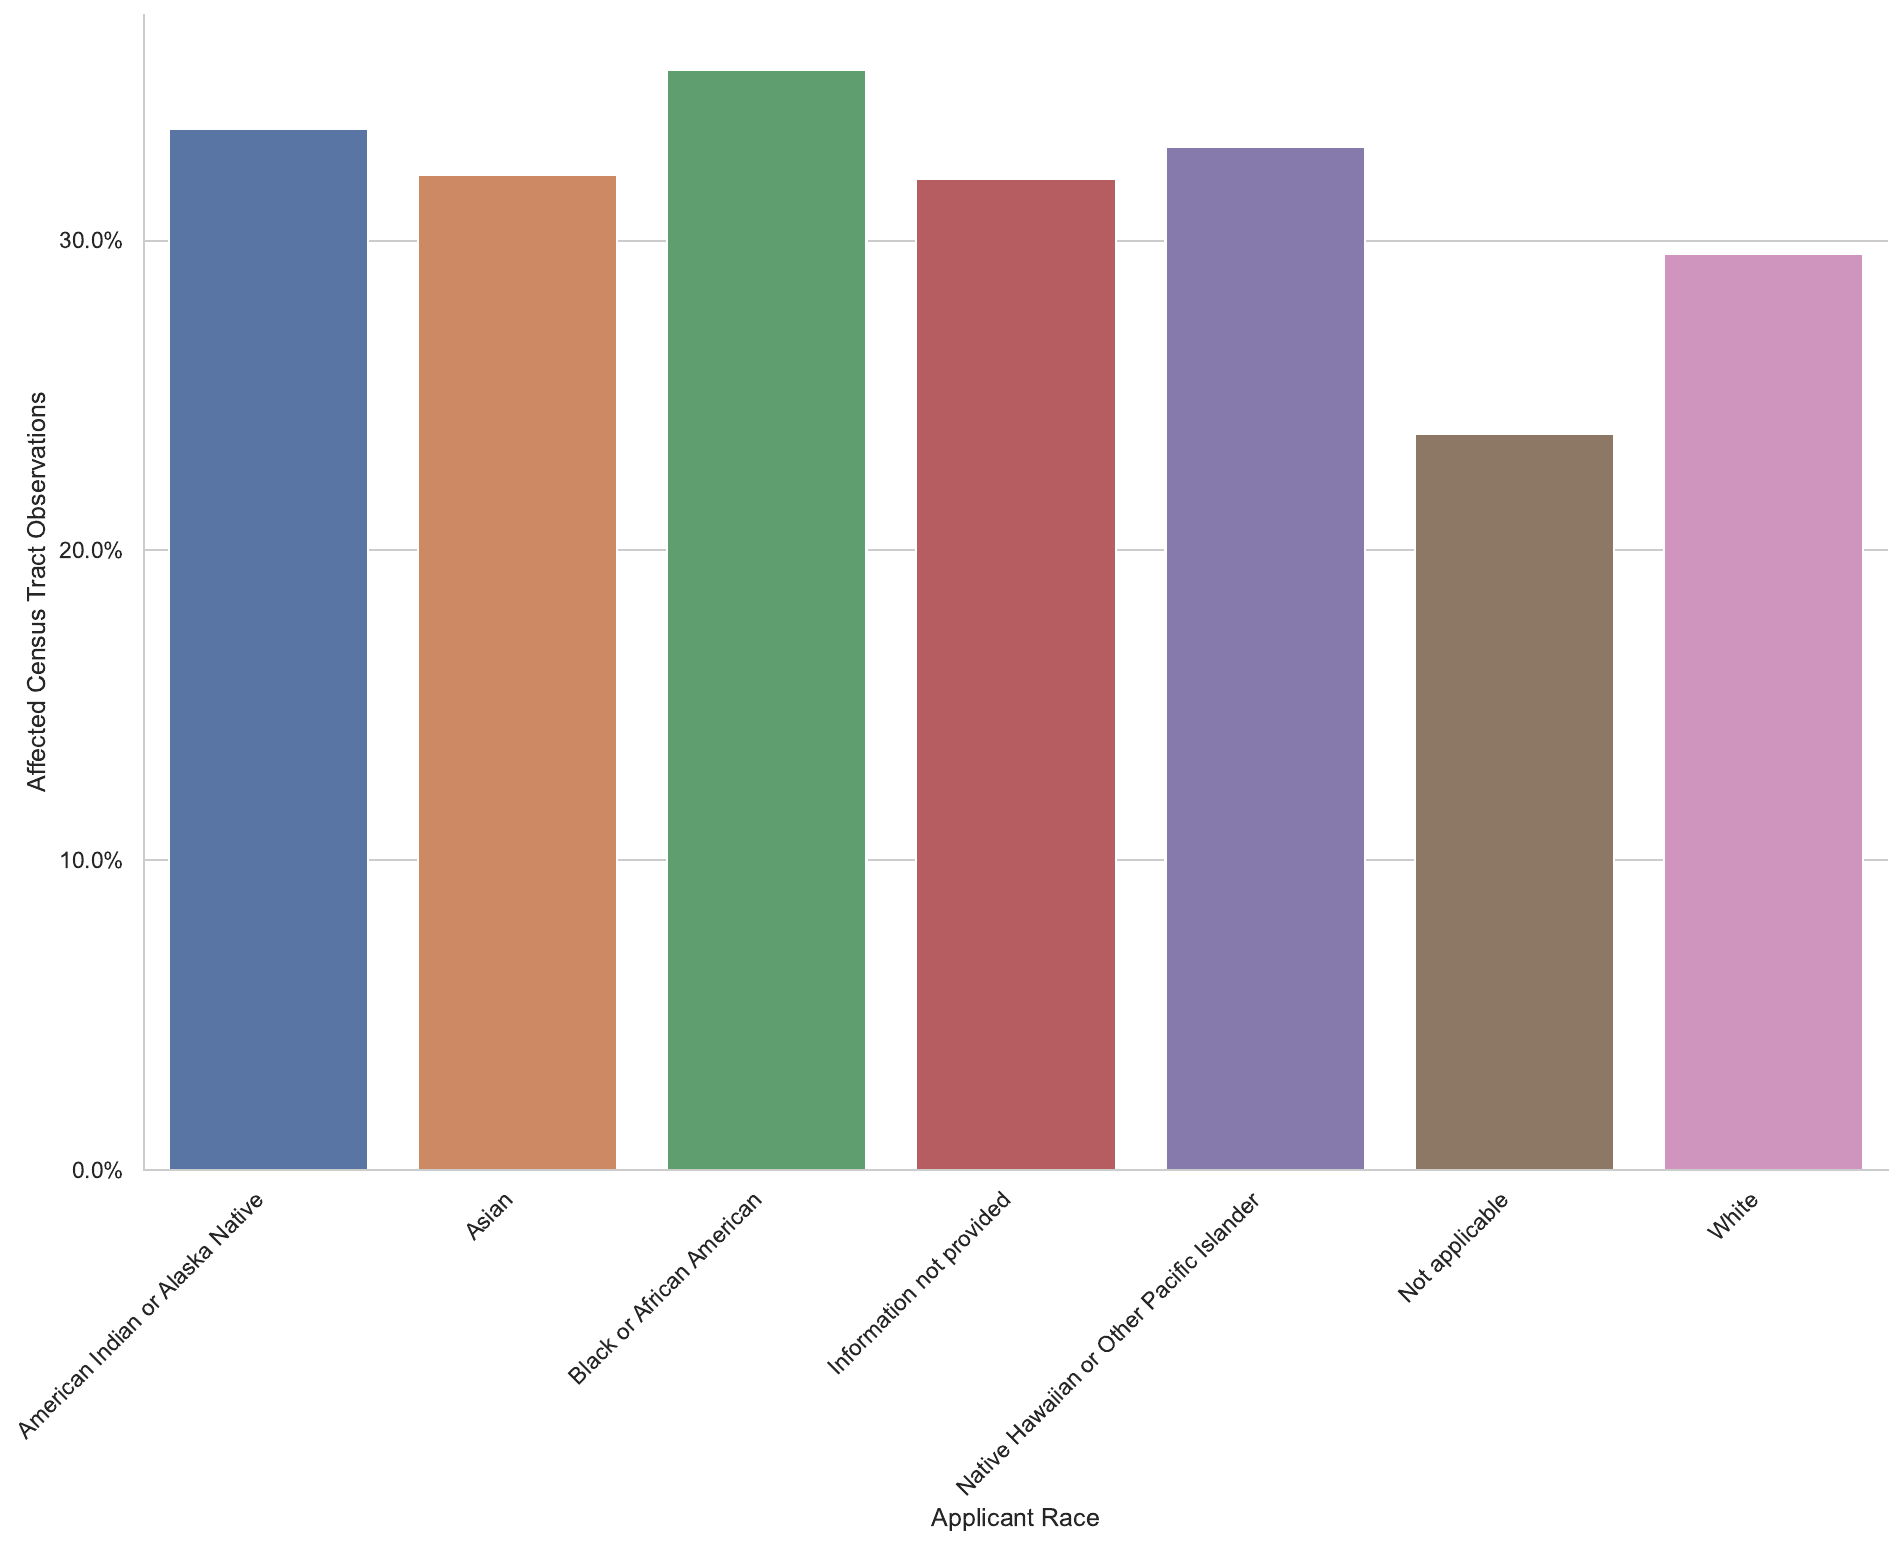}
\caption{}
\end{subfigure}
\caption{Duplicate Observations by (a) Share of Majority Race and (b) Race}\label{fig:deletion_by_majority_share}
\end{center}
\begin{flushleft}
\scriptsize{Notes: This figure illustrates the probability of having an observation deleted during the cleaning and merging of credit report data with HMDA data as a function of (a) the share of the majority race in a given Census Tract and (b) race. Deletions are more common in ZIP codes with more diverse populations.}
\end{flushleft}
\end{figure}

\begin{figure}[ht]
\footnotesize
    \centering
    \begin{subfigure}[b]{0.30\textwidth}
        \includegraphics[width=\textwidth]{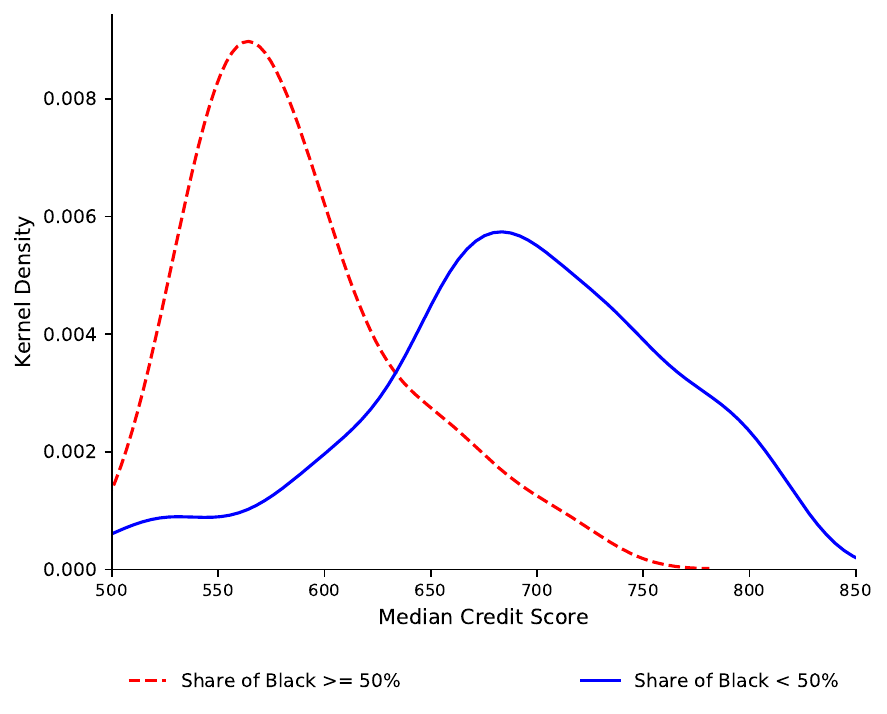}
        \caption{Credit Score}
        \label{fig:cs}
    \end{subfigure}
    \begin{subfigure}[b]{0.30\textwidth}
        \includegraphics[width=\textwidth]{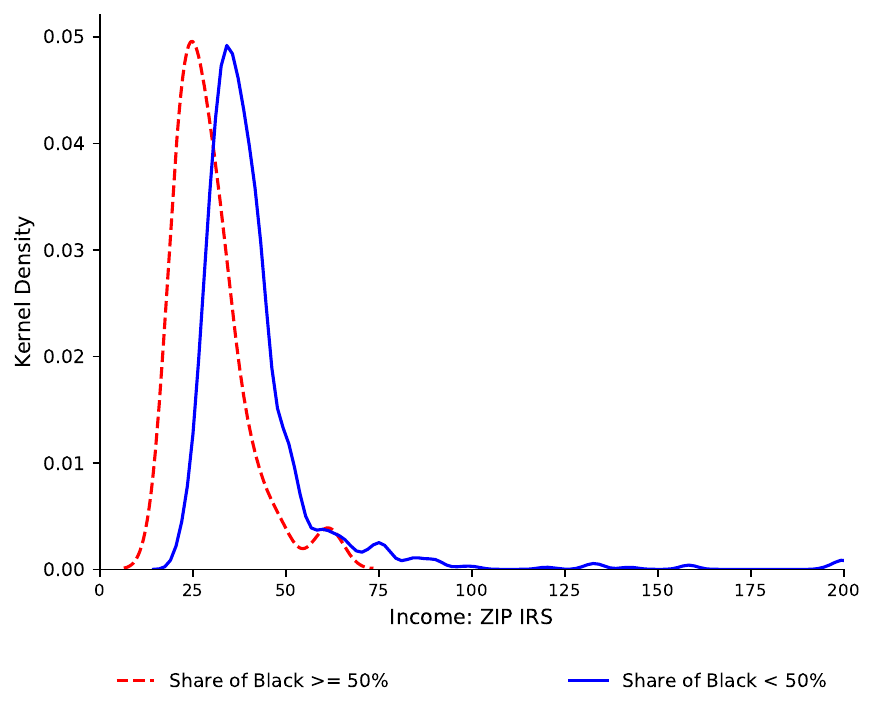}
        \caption{Household Income}
        \label{fig:hi}
    \end{subfigure} \\
    \begin{subfigure}[b]{0.30\textwidth}
        \includegraphics[width=\textwidth]{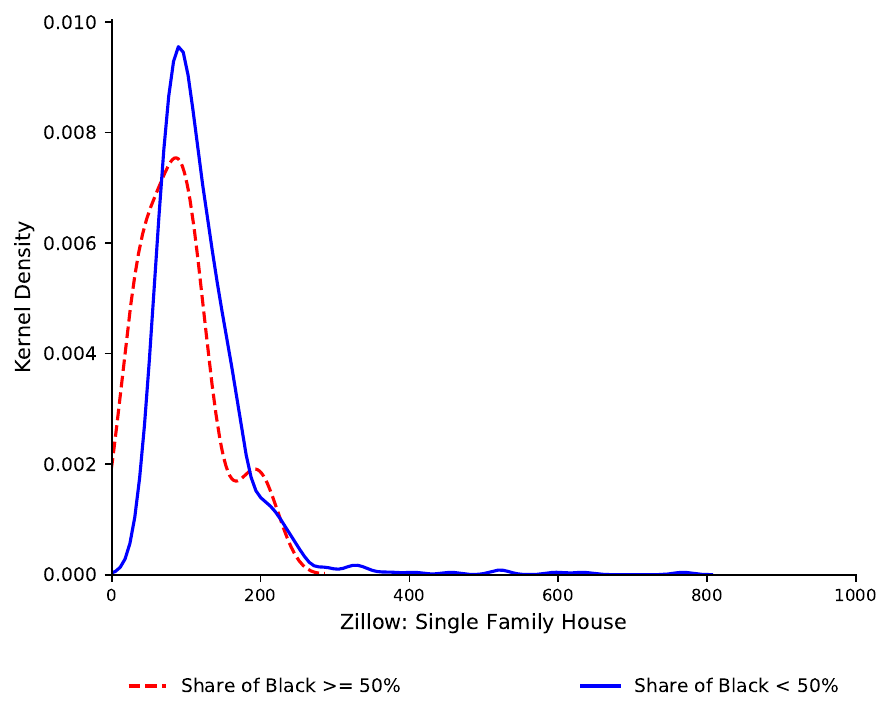}
        \caption{House Value}
        \label{fig:hv}
        \end{subfigure}
     \begin{subfigure}[b]{0.30\textwidth}
        \includegraphics[width=\textwidth]{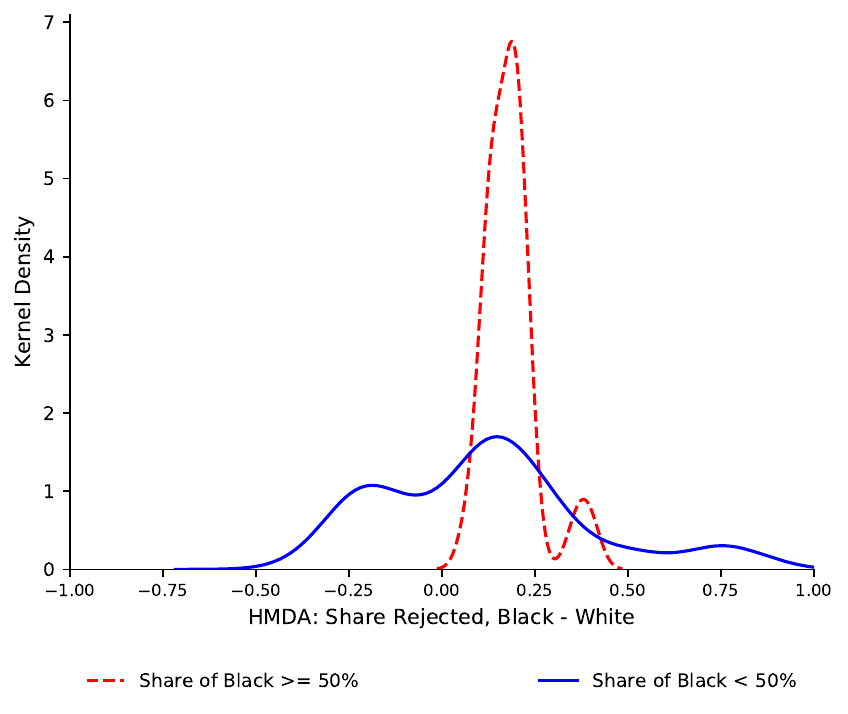}
        \caption{Mortgage Denials}
        \label{fig:hmda}       
    \end{subfigure} \\
        \begin{subfigure}[b]{0.30\textwidth}
        \includegraphics[width=\textwidth]{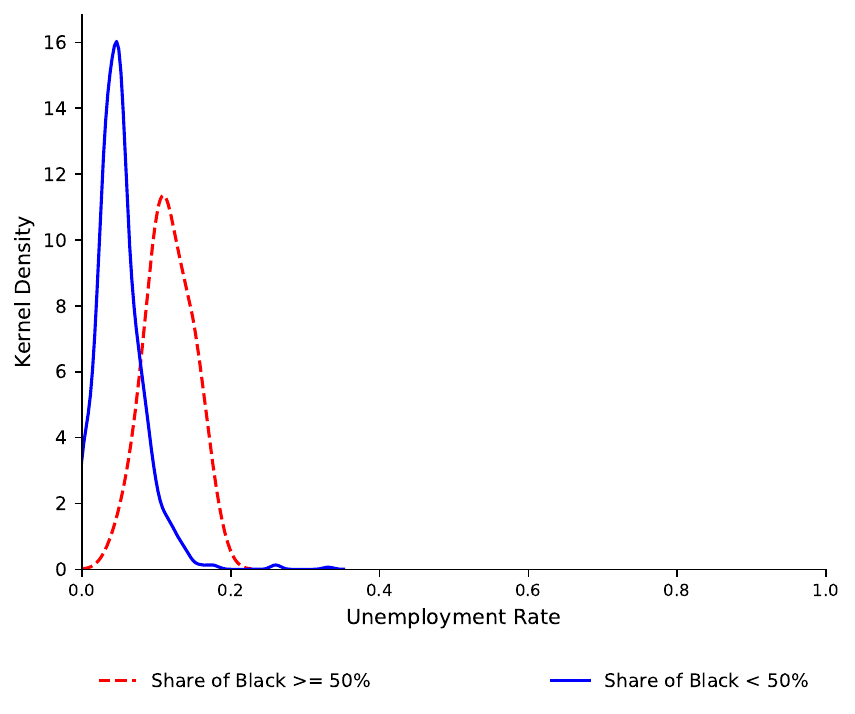}
        \caption{Unemployment Rate}
        \label{fig:ur}
    \end{subfigure}
        \begin{subfigure}[b]{0.30\textwidth}
        \includegraphics[width=\textwidth]{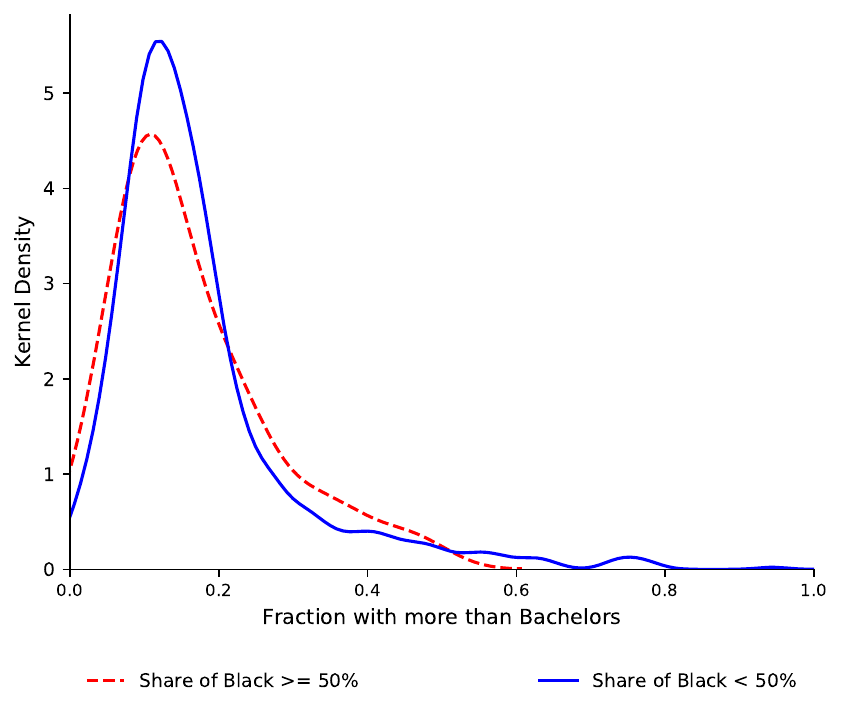}
        \caption{$>=$ Bachelor Degree}
        \label{fig:bd}
    \end{subfigure}
    \caption{Kernel Density Estimates of Selected Covariates}\label{fig:kde}
    \begin{flushleft}
\scriptsize{Notes:  These figures plot the densities of various neighborhood characteristics cross majority black and majority non-black neighborhoods. Data come from the entire Missouri zip code level dataset.}
\end{flushleft} 
\end{figure}

\clearpage 

\subsection*{Appendix Tables}
\begin{table}[htbp]\centering
\begin{threeparttable}
\footnotesize
\caption{Itemized Sample Restrictions: Missouri Data}\label{tab:sample_restrictions}
\begin{tabular}{lcc} \hline \hline
 &  ZIP Codes & \% Black  \\ \hline 
ACS & 1,021 &  4.8\%  
 \\ 
Demographic \& Judgment Information Available  & 1,015 &  4.8\%
 \\ 
Credit Report Information Available  & 902 &  5.5\%
 \\ 
Common Support Sample  & 840 &  5.6\%
 \\ 
 \hline \hline 
\end{tabular}
\begin{tablenotes}
\scriptsize
\item Notes:  This table documents the numbers of zip codes and the average percentage of the population that is black across different samples of data from Missouri.  
\end{tablenotes}
\end{threeparttable}
\end{table}

\begin{table}[htbp] \centering
\begin{threeparttable}
\footnotesize
\def\sym#1{\ifmmode^{#1}\else\(^{#1}\)\fi}
\caption{Judgments, Income, and Credit Scores \label{tab:creditworthiness}}
\begin{tabular}{l*{6}{c}}
\hline\hline
                    &\multicolumn{1}{c}{(1)}&\multicolumn{1}{c}{(2)}&\multicolumn{1}{c}{(3)}&\multicolumn{1}{c}{(4)}&\multicolumn{1}{c}{(5)}&\multicolumn{1}{c}{(6)}\\
                       &\multicolumn{6}{c}{Judgment Rate}\\
\hline
& & & & & & \\[\dimexpr-\normalbaselineskip+2pt]
Black Majority: ZIP &      1.4356\sym{***}&      0.8629\sym{***}&      1.0786\sym{***}&      0.7939\sym{***}&      0.7084\sym{***}&      0.8384\sym{***}\\
                    &    (0.1873)         &    (0.1917)         &    (0.1658)         &    (0.1807)         &    (0.1662)         &    (0.0356)         \\
\hline
& & & & & & \\[\dimexpr-\normalbaselineskip+2pt]

Baseline Controls   &                     &                     &                     &                     &           X         &                     \\
Income      &                     &           X         &                     &           X         &           X         &                     \\
Credit Score    &                     &                     &           X         &           X         &           X         &                     \\
Lagged Baseline Controls&                     &                     &                     &                     &                     &           X         \\
& & & & & & \\[\dimexpr-\normalbaselineskip+2pt] \hline 
Wild Cluster Bootstrap p-value&           0         &           0         &           0         &       .0005         &       .0009         &           0         \\
Observations        &   7365      &   7365      &   7019      &   7019      &   7019      &   6105      \\
$R^2$               &      0.5961         &      0.6617         &      0.6279         &      0.6684         &      0.6851         &      0.6770         \\
\hline\hline
\end{tabular}
\begin{tablenotes}
\scriptsize
\item Notes:  This table presents results of a regression of the judgment rate on neighborhood racial composition and other neighborhood-level characteristics.  The sample includes Missouri zip codes in the common support sample.  The dependent variable is judgments per 100 individuals.  Income controls include average zip code-level income and the fraction of IRS filings under \$25,000, between \$25,000-50,000, \$50,000-75,000, \$75,000-100,000, and over \$100,000; credit controls include credit score quintiles and median credit score; baseline controls include total delinquent debt balances, unemployment rate, median house value, the fraction of the population with a college education, the divorce rate, and population density. All regressions are weighted by population. Robust standard errors clustered at the county-year level are in parentheses. Effective number of clusters: 36.0. Wild Cluster Bootstrap p-values are reported for our main parameter of interest. \sym{*} \(p<0.10\), \sym{**} \(p<0.05\), \sym{***} \(p<0.01\). 
\end{tablenotes}
\end{threeparttable}
\end{table}

\begin{table}[htbp] \centering
\begin{threeparttable}
\footnotesize
\def\sym#1{\ifmmode^{#1}\else\(^{#1}\)\fi}
\caption{Judgments and Plaintiff Type\label{tab:plaintiff_type}}
\begin{tabular}{l*{6}{c}}
\hline\hline
                    &\multicolumn{1}{c}{(1)}&\multicolumn{1}{c}{(2)}&\multicolumn{1}{c}{(3)}&\multicolumn{1}{c}{(4)}&\multicolumn{1}{c}{(5)}&\multicolumn{1}{c}{(6)}\\
                    &\multicolumn{1}{c}{Judgments}&\multicolumn{1}{c}{Debt Buyer}&\multicolumn{1}{c}{Major Bank}&\multicolumn{1}{c}{Medical}&\multicolumn{1}{c}{High-Cost }&\multicolumn{1}{c}{Misc.}\\
\hline
& & & & & & \\[\dimexpr-\normalbaselineskip+2pt]
Black Majority: ZIP &       0.708\sym{***}&       0.217\sym{***}&       0.058\sym{**} &       0.045         &       0.119\sym{***}&       0.321\sym{***}\\
                    &     (0.166)         &     (0.051)         &     (0.029)         &     (0.055)         &     (0.024)         &     (0.082)         \\
\hline
& & & & & & \\[\dimexpr-\normalbaselineskip+2pt]
Mean                &       1.253         & .568       &        .453         &        .297         &        .076         &        .139         \\
Effect Size         &56.5         &        38.2         &        12.8         &        15.1         &       156.3         &         231         \\ \hline
& & & & & & \\[\dimexpr-\normalbaselineskip+2pt]
Wild Cluster Bootstrap p-value&       .0009         &       .0006         &       .0652         &       .5694         &           0         &       .0001         \\
Observations        &    7019        &    7019        &    7019        &    7019        &    7019        &    7019        \\
$R^2$               &       0.685         &       0.699         &       0.725         &       0.613         &       0.602         &       0.533         \\
\hline\hline
\end{tabular}
\begin{tablenotes}
\scriptsize
\item Notes:  This table presents results of a regression of the judgment rate for specific types of debt collectors on neighborhood racial composition and other neighborhood-level characteristics.  The sample includes Missouri zip codes in the common support sample.  The dependent variable in Column (1) is judgments per 100 individuals.  The dependent variables in Columns (2)-(6) are judgements by debt buyers per 100 individuals, judgments by major banks per 100 individuals, judgments by medical lenders per 100 individuals, judgments by high-cost lenders per 100 individuals, and judgments by other miscellaneous lenders per 100 individuals. Baseline controls (average zip code-level income, the fraction of IRS filings under \$25,000, between \$25,000-50,000, \$50,000-75,000, \$75,000-100,000, and over \$100,000, credit score quintiles, median credit score, total delinquent debt balances, unemployment rate, median house value, the fraction of the population with a college education, the divorce rate, and population density), county fixed effects, and year fixed effects are included in all specifications. All regressions are weighted by population. Robust standard errors clustered at the county-year level are in parentheses. Effective number of clusters: 36.0. Wild Cluster Bootstrap p-values are reported for our main parameter of interest. \sym{*} \(p<0.10\), \sym{**} \(p<0.05\), \sym{***} \(p<0.01\). 
\end{tablenotes}
\end{threeparttable}
\end{table}

\begin{table}[htbp] \centering
\begin{threeparttable}
\footnotesize
\def\sym#1{\ifmmode^{#1}\else\(^{#1}\)\fi}
\caption{Judgments and Access to Credit Markets\label{tab:access_to_credit}}
\begin{tabular}{l*{5}{c}}
\hline\hline
                    &\multicolumn{1}{c}{(1)}&\multicolumn{1}{c}{(2)}&\multicolumn{1}{c}{(3)}&\multicolumn{1}{c}{(4)}&\multicolumn{1}{c}{(5)}\\
                       &\multicolumn{5}{c}{Judgment Rate}\\
\hline
& & & & & \\[\dimexpr-\normalbaselineskip+2pt]
Black Majority: ZIP &      1.0910\sym{***}&      1.0897\sym{***}&      1.0914\sym{***}&      0.9375\sym{***}&      0.9417\sym{***}\\
                    &    (0.1398)         &    (0.1394)         &    (0.1399)         &    (0.1099)         &    (0.1135)         \\
& & & & & \\[\dimexpr-\normalbaselineskip+2pt]
Broadband           &                     &      0.0565\sym{**} &                     &                     &                     \\
                    &                     &    (0.0222)         &                     &                     &                     \\
& & & & & \\[\dimexpr-\normalbaselineskip+2pt]
Unscored            &                     &                     &      0.1838         &                     &                     \\
                    &                     &                     &    (0.2691)         &                     &                     \\
& & & & & \\[\dimexpr-\normalbaselineskip+2pt]
Banks (5 miles)     &                     &                     &                     &     -0.0056\sym{***}&                     \\
                    &                     &                     &                     &    (0.0011)         &                     \\
& & & & & \\[\dimexpr-\normalbaselineskip+2pt]
Payday Lenders (5 miles)&                     &                     &                     &      0.0177\sym{***}&                     \\
                    &                     &                     &                     &    (0.0028)         &                     \\
& & & & & \\[\dimexpr-\normalbaselineskip+2pt]
Banks (10 miles)    &                     &                     &                     &                     &     -0.0025\sym{***}\\
                    &                     &                     &                     &                     &    (0.0003)         \\
& & & & & \\[\dimexpr-\normalbaselineskip+2pt]
Payday Lenders (10 miles)&                     &                     &                     &                     &      0.0098\sym{***}\\
                    &                     &                     &                     &                     &    (0.0013)         \\
\hline
& & & & & \\[\dimexpr-\normalbaselineskip+2pt]
Wild Cluster Bootstrap p-value&           0         &           0         &           0         &           0         &           0         \\
\hline 
& & & & & \\[\dimexpr-\normalbaselineskip+2pt]
Observations        &   4183      &   4183      &   4183      &   4183      &   4183      \\
$R^2$               &      0.8181         &      0.8186         &      0.8181         &      0.8279         &      0.8295         \\
\hline\hline
\end{tabular}
\begin{tablenotes}
\scriptsize
\item Notes:  This table presents results of a regression of the judgment rate on neighborhood racial composition and other neighborhood-level characteristics.  The sample includes Missouri zip codes in the common support sample.  The dependent variable is judgments per 100 individuals.  Baseline controls (average zip code-level income, the fraction of IRS filings under \$25,000, between \$25,000-50,000, \$50,000-75,000, \$75,000-100,000, and over \$100,000, credit score quintiles, median credit score, total delinquent debt balances, unemployment rate, median house value, the fraction of the population with a college education, the divorce rate, and population density), county fixed effects, and year fixed effects are included in all specifications. All regressions are weighted by population. Robust standard errors clustered at the county-year level are in parentheses. Effective number of clusters: 36.0. Wild Cluster Bootstrap p-values are reported for our main parameter of interest. \sym{*} \(p<0.10\), \sym{**} \(p<0.05\), \sym{***} \(p<0.01\). 
\end{tablenotes}
\end{threeparttable}
\end{table}

\begin{table}[htbp] \centering
\begin{threeparttable}
\footnotesize 
\def\sym#1{\ifmmode^{#1}\else\(^{#1}\)\fi}
\caption{Judgments and an Alternative Credit Score\label{tab:pp}}
\begin{tabular}{l*{5}{c}}
\hline\hline
                    &\multicolumn{1}{c}{(1)}&\multicolumn{1}{c}{(2)}&\multicolumn{1}{c}{(3)}&\multicolumn{1}{c}{(4)}&\multicolumn{1}{c}{(5)}\\
                       &\multicolumn{5}{c}{Judgment Rate}\\
\hline
& & & & &  \\[\dimexpr-\normalbaselineskip+2pt]
Black Majority: ZIP &      1.6061\sym{***}&      1.2321\sym{***}&      0.9537\sym{***}&      0.8287\sym{***}&      1.0213\sym{***}\\
                    &    (0.1885)         &    (0.1717)         &    (0.1961)         &    (0.1764)         &    (0.0360)         \\
\hline
& & & & &  \\[\dimexpr-\normalbaselineskip+2pt]
Baseline Controls   &                     &                     &                     &           X         &                     \\
Income              &                     &                     &           X         &           X         &                     \\
Default Probability &                     &           X         &           X         &           X         &           X         \\
Lagged Baseline Controls&                     &                     &                     &                     &           X         \\
\hline
& & & & &  \\[\dimexpr-\normalbaselineskip+2pt]
Wild Cluster Bootstrap p-value&           0         &           0         &       .0001         &       .0007         &           0         \\
Observations        &   5909      &   5909      &   5909      &   5625      &   4738      \\
$R^2$               &      0.5977         &      0.6319         &      0.6813         &      0.7001         &      0.7291         \\
\hline\hline
\end{tabular}
\begin{tablenotes}
\scriptsize
\item Notes:  This table presents results of a regression of the judgment rate on neighborhood racial composition and other neighborhood-level characteristics.  The sample includes Missouri zip codes in the common support sample.  The dependent variable is judgments per 100 individuals.  Baseline controls (average zip code-level income, the fraction of IRS filings under \$25,000, between \$25,000-50,000, \$50,000-75,000, \$75,000-100,000, and over \$100,000, total delinquent debt balances, unemployment rate, median house value, the fraction of the population with a college education, the divorce rate, and population density), county fixed effects, and year fixed effects are included in all specifications. Default probabilities are used as control variables in place of credit scores. Column (5) controls for lagged default probability instead of default probability. Default probability data is available starting in 2006. All regressions are weighted by population. Robust standard errors clustered at the county-year level are in parentheses. Effective number of clusters: 36.0. Wild Cluster Bootstrap p-values are reported for our main parameter of interest. \sym{*} \(p<0.10\), \sym{**} \(p<0.05\), \sym{***} \(p<0.01\). 
\end{tablenotes}
\end{threeparttable}
\end{table}

\begin{table}[htbp] \centering
\begin{threeparttable}
\footnotesize
\def\sym#1{\ifmmode^{#1}\else\(^{#1}\)\fi}
\caption{Judgments and Local Housing Markets\label{tab:access_to_housing}}
\begin{tabular}{l*{4}{c}}
\hline\hline
                    &\multicolumn{1}{c}{(1)}&\multicolumn{1}{c}{(2)}&\multicolumn{1}{c}{(3)}&\multicolumn{1}{c}{(4)}\\
                       &\multicolumn{4}{c}{Judgment Rate}\\
\hline
& & & & \\[\dimexpr-\normalbaselineskip+2pt]
Black Majority: ZIP &      0.9451\sym{***}&      0.8416\sym{***}&      0.7136\sym{***}&      0.6891\sym{***}\\
                    &    (0.1581)         &    (0.1453)         &    (0.1610)         &    (0.1584)         \\
& & & & \\[\dimexpr-\normalbaselineskip+2pt]
HMDA: Share Rejected&                     &      1.0981\sym{***}&                     &                     \\
                    &                     &    (0.3638)         &                     &                     \\
& & & & \\[\dimexpr-\normalbaselineskip+2pt]
Zillow: Single Family House&                     &                     &                     &     -0.0060\sym{***}\\
                    &                     &                     &                     &    (0.0013)         \\
\hline
& & & & \\[\dimexpr-\normalbaselineskip+2pt]
HMDA Available      &           X         &           X         &                     &                     \\
Zillow Available    &                     &                     &           X         &           X         \\ \hline
& & & & \\[\dimexpr-\normalbaselineskip+2pt]
Wild Cluster Bootstrap p-value&           0         &           0         &       .0006         &       .0005         \\
Observations        &   3846         &   3846         &   5231         &   5231         \\
$R^2$               &      0.7593         &      0.7628         &      0.6767         &      0.6861         \\
\hline\hline
\end{tabular}
\begin{tablenotes}
\scriptsize
\item Notes:  This table presents results of a regression of the judgment rate on neighborhood racial composition and other neighborhood-level characteristics, including information on local housing markets.  The sample includes Missouri zip codes in the common support sample.  The dependent variable is judgments per 100 individuals.  Baseline controls (average zip code-level income, the fraction of IRS filings under \$25,000, between \$25,000-50,000, \$50,000-75,000, \$75,000-100,000, and over \$100,000, credit score quintiles, median credit score, total delinquent debt balances, unemployment rate, median house value, the fraction of the population with a college education, the divorce rate, and population density), county fixed effects, and year fixed effects are included in all specifications.  All regressions are weighted by population. Robust standard errors clustered at the county-year level are in parentheses. Effective number of clusters: 36.0. Wild Cluster Bootstrap p-values are reported for our main parameter of interest. \sym{*} \(p<0.10\), \sym{**} \(p<0.05\), \sym{***} \(p<0.01\). 
\end{tablenotes}
\end{threeparttable}
\end{table}

\begin{sidewaystable}[htbp] \centering
\begin{threeparttable}
\footnotesize
\def\sym#1{\ifmmode^{#1}\else\(^{#1}\)\fi}
\caption{Judgments and Alternative Dependent Variables\label{tab:judgment_alternative}}
\begin{tabular}{l*{7}{c}}
\hline\hline
                    &\multicolumn{1}{c}{(1)}&\multicolumn{1}{c}{(2)}&\multicolumn{1}{c}{(3)}&\multicolumn{1}{c}{(4)}&\multicolumn{1}{c}{(5)}&\multicolumn{1}{c}{(6)}&\multicolumn{1}{c}{(7)}\\
&\multicolumn{1}{c}{Judgments/Cases}&\multicolumn{2}{c}{Judgment: Low Income}&\multicolumn{2}{c}{Judgment: Low Credit }&\multicolumn{2}{c}{Judgment: Winsorized} \\
\hline
& & & & & &  \\[\dimexpr-\normalbaselineskip+2pt]
Black Majority: ZIP &    0.028\sym{***} &       2.843\sym{***}&       2.649\sym{***}&       0.503\sym{***}&       0.492\sym{***} &      0.708\sym{***}&       0.666\sym{***}\\
              &     (0.010)                   &     (0.704)         &     (0.570)         &     (0.122)         &     (0.115)     &     (0.165)         &     (0.138)         \\
\hline
& & & & & &  \\[\dimexpr-\normalbaselineskip+2pt]
Population Weighted &                   &             X       &                  &                X     &                 &          X           &                     \\
\hline
& & & & & &  \\[\dimexpr-\normalbaselineskip+2pt]
Wild Cluster Boostrap p-value   &       .0111        &       .0011         &           0         &        .003         &       .0005          &       .0008         &       .0002       \\
Observations        &    7019         &    7019         &    7019              &    6999         &    6999      &    7019       &    7019         \\
$R^2$         &       0.173                &       0.660         &       0.548         &       0.744         &       0.576         &       0.686         &       0.512        \\
\hline\hline
\end{tabular}
\begin{tablenotes}
\scriptsize
\item  Notes:  This table presents results of a regression of the judgment rate on neighborhood racial composition and other neighborhood-level characteristics, where the judgment rate is normalized in various ways.  The sample includes Missouri zip codes in the common support sample.  For Column (1) our dependent variable is the fraction of cases that result in a judgment, for Columns (2-3), our outcome variable is judgments per 100 individuals with tax filings under \$25,000 USD, for Columns (4-5) our outcome variable is judgments per 100 individuals with subprime credit, and for Columns (6-7) we winsorize our main outcome variable, judgments per 100 individuals, at the 99th percentile. Baseline controls (average zip code-level income, the fraction of IRS filings under \$25,000, between \$25,000-50,000, \$50,000-75,000, \$75,000-100,000, and over \$100,000, credit score quintiles, median credit score, total delinquent debt balances, unemployment rate, median house value, the fraction of the population with a college education, the divorce rate, and population density), county fixed effects, year fixed effects, and attorney representation are included in all specifications.  Only columns (2), (4), and (6) are weighted by population. Robust standard errors clustered at the county-year level are in parentheses. Effective number of clusters: 36.0. Wild Cluster Bootstrap p-values are reported for our main parameter of interest. \sym{*} \(p<0.10\), \sym{**} \(p<0.05\), \sym{***} \(p<0.01\). 
\end{tablenotes}
\end{threeparttable}
\end{sidewaystable}

\begin{table}[htbp] \centering
\begin{threeparttable}
\footnotesize
\def\sym#1{\ifmmode^{#1}\else\(^{#1}\)\fi}
\caption{Judgments and an Alternative Proxy for Race\label{tab:race_proxies}}
\begin{tabular}{l*{4}{c}}
\hline\hline
                    &\multicolumn{1}{c}{(1)}&\multicolumn{1}{c}{(2)}&\multicolumn{1}{c}{(3)}&\multicolumn{1}{c}{(4)}\\
                       &\multicolumn{4}{c}{Judgment Rate}\\
\hline
& & &  & \\[\dimexpr-\normalbaselineskip+2pt]
Share Black: ZIP    &      1.4731\sym{***}&                     &                     &                     \\
                    &    (0.2865)         &                     &                     &                     \\
& & &  & \\[\dimexpr-\normalbaselineskip+2pt]
Black Majority: ZIP &                     &      0.7084\sym{***}&                     &                     \\
                    &                     &    (0.1662)         &                     &                     \\
& & &  & \\[\dimexpr-\normalbaselineskip+2pt]
Share Black: BISG   &                     &                     &      1.3776\sym{***}&                     \\
                    &                     &                     &    (0.2563)         &                     \\
& & &  & \\[\dimexpr-\normalbaselineskip+2pt]
Black Majority: BISG&                     &                     &                     &      0.6283\sym{***}\\
                    &                     &                     &                     &    (0.1347)         \\
\hline
& & &  & \\[\dimexpr-\normalbaselineskip+2pt]
Wild Cluster Bootstrap p-value&       .0001         &       .0009         &           0         &       .0005         \\
Observations        &   7019         &   7019         &   7015         &   7015         \\
$R^2$               &      0.6965         &      0.6851         &      0.6981         &      0.6860         \\
\hline\hline
\end{tabular}
\begin{tablenotes}
\scriptsize
\item Notes:  This table presents results of a regression of the judgment rate on neighborhood racial composition (where racial composition is measured in various ways) and other neighborhood-level characteristics.  The sample includes Missouri zip codes in the common support sample.  The dependent variable is judgments per 100 individuals.  Baseline controls (average zip code-level income, the fraction of IRS filings under \$25,000, between \$25,000-50,000, \$50,000-75,000, \$75,000-100,000, and over \$100,000, credit score quintiles, median credit score, total delinquent debt balances, unemployment rate, median house value, the fraction of the population with a college education, the divorce rate, and population density), county fixed effects, and year fixed effects are included in all specifications.  All regressions are weighted by population. Robust standard errors clustered at the county-year level are in parentheses. Effective number of clusters: 36.0. Wild Cluster Bootstrap p-values are reported for our main parameter of interest. \sym{*} \(p<0.10\), \sym{**} \(p<0.05\), \sym{***} \(p<0.01\). 
\end{tablenotes}
\end{threeparttable}
\end{table}

\begin{table}[htbp] \centering
\begin{threeparttable}
\footnotesize
\def\sym#1{\ifmmode^{#1}\else\(^{#1}\)\fi}
\caption{Judgments and Debt Portfolios: Share Black\label{tab:debt_composition_share_black}}
\begin{tabular}{l*{5}{c}}
\hline\hline
                    &\multicolumn{1}{c}{(1)}&\multicolumn{1}{c}{(2)}&\multicolumn{1}{c}{(3)}&\multicolumn{1}{c}{(4)}&\multicolumn{1}{c}{(5)}\\
                       &\multicolumn{5}{c}{Judgment Rate}\\
\hline
& & & & & \\[\dimexpr-\normalbaselineskip+2pt]
Share Black: ZIP    &      1.4651\sym{***}&      1.4758\sym{***}&      1.4727\sym{***}&      1.5054\sym{***}&      1.4915\sym{***}\\
                    &    (0.2789)         &    (0.2851)         &    (0.2850)         &    (0.2750)         &    (0.2655)         \\
\hline
& & & & & \\[\dimexpr-\normalbaselineskip+2pt]
Debt Levels         &           X         &                     &                     &                     &           X         \\
Monthly Payment and Utilization&                     &           X         &                     &                     &           X         \\
Debt Composition    &                     &                     &           X         &                     &           X         \\
Delinquency/Bankruptcy/Collections&                     &                     &                     &           X         &           X         \\
\hline
& & & & & \\[\dimexpr-\normalbaselineskip+2pt]
Wild Cluster Bootstrap p-value&           0         &       .0001         &           0         &           0         &           0         \\
Observations        &   7019        &   7019        &   7019        &   7019        &   7019        \\
$R^2$               &      0.6995         &      0.6973         &      0.6968         &      0.6995         &      0.7045         \\
\hline\hline
\end{tabular}
\begin{tablenotes}
\scriptsize
\item Notes:  This table presents results of a regression of the judgment rate on neighborhood racial composition (as measured by the share of black residents) and other neighborhood-level characteristics.  The sample includes Missouri zip codes in the common support sample.  The dependent variable is judgments per 100 individuals.  Baseline controls (average zip code-level income, the fraction of IRS filings under \$25,000, between \$25,000-50,000, \$50,000-75,000, \$75,000-100,000, and over \$100,000, credit score quintiles, median credit score, total delinquent debt balances, unemployment rate, median house value, the fraction of the population with a college education, the divorce rate, and population density), county fixed effects, and year fixed effects are included in all specifications.  All regressions are weighted by population. Robust standard errors clustered at the county-year level are in parentheses. Effective number of clusters: 36.0. Wild Cluster Bootstrap p-values are reported for our main parameter of interest. \sym{*} \(p<0.10\), \sym{**} \(p<0.05\), \sym{***} \(p<0.01\). 
\end{tablenotes}
\end{threeparttable}
\end{table}

\begin{sidewaystable}[htbp]\centering
\begin{threeparttable}
\footnotesize
\def\sym#1{\ifmmode^{#1}\else\(^{#1}\)\fi}
\caption{Attorney Representation and Judgment Type: Share Black\label{tab:judgment_type_share_black}}
\begin{tabular}{l*{8}{c}}
\hline\hline
                    &\multicolumn{1}{c}{(1)}&\multicolumn{1}{c}{(2)}&\multicolumn{1}{c}{(3)}&\multicolumn{1}{c}{(4)}&\multicolumn{1}{c}{(5)}&\multicolumn{1}{c}{(6)}&\multicolumn{1}{c}{(7)}&\multicolumn{1}{c}{(8)}\\
                    &\multicolumn{1}{c}{Attorney}&\multicolumn{1}{c}{Judgments}&\multicolumn{1}{c}{Consent}&\multicolumn{1}{c}{Constested}&\multicolumn{1}{c}{Default}&\multicolumn{1}{c}{Dismissed}&\multicolumn{1}{c}{Settle}&\multicolumn{1}{c}{Judgments}\\
\hline
&&&&& & & & \\[\dimexpr-\normalbaselineskip+2pt]
Share Black: ZIP    &      -0.036\sym{***}&       1.409\sym{***}&       1.474\sym{***}&       0.014         &       0.011\sym{*}  &       0.045\sym{***}&       0.010         &      1.575\sym{***}\\
                    &     (0.006)         &     (0.282)         &     (0.283)         &     (0.011)         &     (0.006)         &     (0.009)         &     (0.011)         &     (0.289)         \\
\hline
&&&&& & & & \\[\dimexpr-\normalbaselineskip+2pt]
Attorney Representation & & X & X&X&X&X&X&X \\
Lagged Case Outcomes & & & & & & & & X \\ \hline 
&&&&& & & & \\[\dimexpr-\normalbaselineskip+2pt]
Wild Cluster Bootstrap p-value&           0         &       .0002         &           0         &       .2137         &       .0987         &           0         &       .3535         &           0.0001         \\
Observations        &    7019      &    7019      &    7019      &    7019      &    7019      &    7019      &    7019      &    6093     \\
$R^2$               &       0.450         &       0.710         &       0.697         &       0.470         &       0.438         &       0.397         &       0.650         &       0.730         \\
\hline\hline
\end{tabular}
\begin{tablenotes}
\scriptsize
\item Notes:  This table explores the extent to which attorney representation or previous case outcomes can explain the racial gap in judgments, using the share of black residents in a zip code as our measure for racial composition.  The sample includes Missouri zip codes in the common support sample. The outcome variable in Column (1) is the share of debt collection court cases where an attorney represented the defendant.  The outcome variable in columns (2) and (8) are judgments per 100 people.  The outcome variables in Columns (3)-(7) are the share of cases resulting in a consent judgment, a contested judgment, a default judgment, the case being dismissed, and the case being settled, respectively.  All regressions are weighted by population. Baseline controls (average zip code-level income, the fraction of IRS filings under \$25,000, between \$25,000-50,000, \$50,000-75,000, \$75,000-100,000, and over \$100,000, credit score quintiles, median credit score, total delinquent debt balances, unemployment rate, median house value, the fraction of the population with a college education, the divorce rate, and population density), county fixed effects, and year fixed effects are included in all specifications. Aside from Column (1), all specifications control for the share of cases with attorney representation. Column (8) controls for the share of default judgments. Robust standard errors clustered at the county-year level are in parentheses. Effective number of clusters: 28.0. Wild Cluster Bootstrap p-values are reported for our main parameter of interest. \sym{*} \(p<0.10\), \sym{**} \(p<0.05\), \sym{***} \(p<0.01\). 
\end{tablenotes}
\end{threeparttable}
\end{sidewaystable}

\begin{table}[htbp]\centering
\begin{threeparttable}
\footnotesize
\def\sym#1{\ifmmode^{#1}\else\(^{#1}\)\fi}
\caption{Debt Portfolios\label{tab:debt_composition_bisg}}
\begin{tabular}{l*{5}{c}}
\hline\hline
                    &\multicolumn{1}{c}{(1)}&\multicolumn{1}{c}{(2)}&\multicolumn{1}{c}{(3)}&\multicolumn{1}{c}{(4)}&\multicolumn{1}{c}{(5)}\\
                       &\multicolumn{5}{c}{Judgment Rate}\\
\hline
Black Majority: BISG&      0.6222\sym{***}&      0.6329\sym{***}&      0.6264\sym{***}&      0.6302\sym{***}&      0.6266\sym{***}\\
                    &    (0.1308)         &    (0.1349)         &    (0.1343)         &    (0.1274)         &    (0.1229)         \\
\hline
Debt Levels         &           X         &                     &                     &                     &           X         \\
Monthly Payment and Utilization&                     &           X         &                     &                     &           X         \\
Debt Composition    &                     &                     &           X         &                     &           X         \\
Delinquency/Bankruptcy/Collections&                     &                     &                     &           X         &           X         \\
Wild Cluster Bootstrap p-value&       .0004         &       .0004         &       .0005         &       .0002         &       .0002         \\
Observations        &   7015       &   7015        &   7015      &   7015        &   7015        \\
$R^2$               &      0.6893         &      0.6869         &      0.6861         &      0.6884         &      0.6940         \\
\hline\hline
\end{tabular}
\begin{tablenotes}
\scriptsize
\item  This table presents results of a regression of the judgment rate on neighborhood racial composition (as defined using the BISG algorithm) and other neighborhood-level characteristics.  The sample includes Missouri zip codes in the common support sample.  The dependent variable is judgments per 100 individuals.  Baseline controls include average zip code-level income, the fraction of IRS filings under \$25,000, between \$25,000-50,000, \$50,000-75,000, \$75,000-100,000, and over \$100,000, credit score quintiles, median credit score, total delinquent debt balances, unemployment rate, median house value, the fraction of the population with a college education, the divorce rate, and population density.  Baseline controls, county fixed effects, and year fixed effects are included in all specifications, and all regressions are weighted by population. Robust standard errors clustered at the county-year level are in parentheses. Effective number of clusters: 36.0. Wild Cluster Bootstrap p-values are reported for our main parameter of interest. \sym{*} \(p<0.10\), \sym{**} \(p<0.05\), \sym{***} \(p<0.01\). 
\end{tablenotes}
\end{threeparttable}
\end{table}

\begin{table}[b]
\centering
\begin{threeparttable}
\footnotesize
\def\sym#1{\ifmmode^{#1}\else\(^{#1}\)\fi}
\caption{Summary Statistics: IL \& NJ\label{tab:summary_statistics_il_nj}}
\begin{tabular}{l*{3}{cc}}
\hline\hline
                    &\multicolumn{1}{c}{Black}&\multicolumn{1}{c}{Non-Black}&\multicolumn{1}{c}{Difference}\\
\hline
& & & \\[\dimexpr-\normalbaselineskip+2pt]
\textbf{Panel A: Judgments and Financial Characteristics} & & & \\
 \textcolor{white}{...}Judgments per 100 People &        2.70&        1.72&       -0.98\sym{***}\\
                    &      (2.00)&      (1.79)&                     \\
 \textcolor{white}{...}Median Credit Score  &      588.98&      707.15&      118.17\sym{***}\\
                    &     (36.72)&     (54.62)&                     \\
 \textcolor{white}{...}90+ DPD Debt Balances &     7135.13&     4260.03&    -2875.10\sym{***}\\
                    &   (6609.97)&   (6448.52)&                     \\
\textbf{Panel B: Additional Neighborhood Characteristics } & & & \\ 
 \textcolor{white}{...}GINI Index       &        0.46&        0.41&       -0.06\sym{***}\\
                    &      (0.05)&      (0.05)&                     \\
 \textcolor{white}{...}Unemployment Rate  &        0.12&        0.07&       -0.06\sym{***}\\
                    &      (0.03)&      (0.02)&                     \\
 \textcolor{white}{...}Divorce Rate  &        0.11&        0.10&       -0.02\sym{***}\\
                    &      (0.02)&      (0.03)&                     \\
 \textcolor{white}{...}Fraction with Bachelors Degree&        0.18&        0.30&        0.11\sym{***}\\
                    &      (0.10)&      (0.14)&                     \\
 \textcolor{white}{...}Gross Rent: Median   &        0.97&        1.06&        0.09\sym{***}\\
                    &      (0.25)&      (0.29)&                     \\
 \textcolor{white}{...}Home Ownership Rate      &        0.51&        0.71&        0.20\sym{***}\\
                    &      (0.20)&      (0.17)&                     \\
 \textcolor{white}{...}Banks (5 miles)  &      166.92&      113.30&      -53.63\sym{***}\\
                    &    (138.48)&    (170.14)&                     \\
 \textcolor{white}{...}Payday Lenders (5 miles)&       33.65&       11.84&      -21.81\sym{***}\\
                    &     (39.86)&     (25.73)&                     \\
 \textcolor{white}{...}Zillow: Single Family House&        176.37&      189.89&       13.53         \\
                    &     (92.22)&    (116.21)&                     \\
 \textcolor{white}{...}HMDA: Share Rejected, Black - White  &      175.91&      252.34&       76.43\sym{***}\\
                    &     (90.21)&    (123.72)&                     \\
 \textcolor{white}{...}Mean Household Income (IRS) &        0.16&        0.13&       -0.03\sym{***}\\
                    &      (0.11)&      (0.19)&                     \\
\hline
Observations        &         200&         705&         905         \\
\hline\hline
\end{tabular}
\begin{tablenotes}
        \scriptsize
        \item Notes:  This table presents summary statistics for the Illinois and New Jersey neighborhood level data from 2004-2013.  The sample includes only observations on the common support.  Column 1 displays the sample means and standard deviations for neighborhoods in which at least 50\% of the population is black and column 2 displays sample means and standard deviations for neighborhoods in which less than 50\% is black.  The third column reports the difference in means across the two samples. \sym{*} \(p<0.10\), \sym{**} \(p<0.05\), \sym{***} \(p<0.01\)
\end{tablenotes}
\end{threeparttable}
\end{table}
\begin{table}[htbp]\centering
\begin{threeparttable}
\footnotesize
\def\sym#1{\ifmmode^{#1}\else\(^{#1}\)\fi}
\caption{Debt Portfolios (NJ and IL Data)\label{tab:debt_composition_nj_il}}
\begin{tabular}{l*{5}{c}}
\hline\hline
                    &\multicolumn{1}{c}{(1)}&\multicolumn{1}{c}{(2)}&\multicolumn{1}{c}{(3)}&\multicolumn{1}{c}{(4)}&\multicolumn{1}{c}{(5)}\\
                       &\multicolumn{5}{c}{Judgment Rate}\\
  
\hline
Black Majority:  ZIP     &      0.2748\sym{***}&      0.2753\sym{***}&      0.2876\sym{***}&      0.2840\sym{***}&      0.2592\sym{***}\\
                    &    (0.0858)         &    (0.0850)         &    (0.0871)         &    (0.0924)         &    (0.0870)         \\
\hline
Wild Cluster Bootstrap p-value&       .0012         &       .0011         &       .0012         &       .0018         &       .0033         \\
Debt Levels         &           X         &                     &                     &                     &           X         \\
Monthly Payment and Utilization&                     &           X         &                     &                     &           X         \\
Debt Composition    &                     &                     &           X         &                     &           X         \\
Delinquency/Bankruptcy/Collections&                     &                     &                     &           X         &           X         \\
Observations        &   3103        &   3103        &   3103        &   3103        &   3103        \\
$R^2$               &      0.9105         &      0.9113         &      0.9101         &      0.9110         &      0.9145         \\
\hline\hline
\end{tabular}
\begin{tablenotes}
\scriptsize
\item Notes:  This table presents results of a regression of the judgment rate on neighborhood racial composition and other neighborhood-level characteristics.  The sample includes New Jersey and Illinois zip codes in the common support sample.  The dependent variable is judgments per 100 individuals.  Baseline controls include average zip code-level income, the fraction of IRS filings under \$25,000, between \$25,000-50,000, \$50,000-75,000, \$75,000-100,000, and over \$100,000, credit score quintiles, median credit score, total delinquent debt balances, unemployment rate, median house value, the fraction of the population with a college education, the divorce rate, and population density.  Baseline controls, county fixed effects, and year fixed effects are included in all specifications, and all regressions are weighted by population. Robust standard errors clustered at the county-year level are in parentheses. Effective number of clusters: 36.0. Wild Cluster Bootstrap p-values are reported for our main parameter of interest. \sym{*} \(p<0.10\), \sym{**} \(p<0.05\), \sym{***} \(p<0.01\). 
\end{tablenotes}
\end{threeparttable}
\end{table}

\begin{table}[b]\centering
  \begin{threeparttable}
 \footnotesize
\def\sym#1{\ifmmode^{#1}\else\(^{#1}\)\fi}
\caption{Summary Statistics: Entire Sample\label{tab:summary_statistics_off_common}}
\begin{tabular}{l*{3}{cc}}
\hline\hline
                    &\multicolumn{1}{c}{Black}&\multicolumn{1}{c}{Non-Black}&\multicolumn{1}{c}{Difference}\\
\hline
& & & \\[\dimexpr-\normalbaselineskip+2pt]
\textbf{Panel A: Judgments and Finacial Characteristics} & & & \\
 \textcolor{white}{...}Judgments per 100 People      &        2.65&        1.32&       -1.32\sym{***}\\
                    &      (1.35)&      (1.53)&                     \\
 \textcolor{white}{...}Share of Default Judgments     &        0.45&        0.37&       -0.08\sym{***}\\
                    &      (0.07)&      (0.17)&                     \\
 \textcolor{white}{...}Share of Consent Judgments          &        0.16&        0.17&        0.02\sym{***}\\
                    &      (0.07)&      (0.14)&                     \\
 \textcolor{white}{...}Share of Dismissed Judgments    &        0.12&        0.15&        0.03\sym{***}\\
                    &      (0.11)&      (0.15)&                     \\
 \textcolor{white}{...}Share of  Constested Judgments        &        0.05&        0.05&       -0.01\sym{*}  \\
                    &      (0.05)&      (0.09)&                     \\
 \textcolor{white}{...}Share of  Settled Cases        &        0.19&        0.21&        0.02\sym{***}\\
                    &      (0.09)&      (0.17)&                     \\
 \textcolor{white}{...}Share w/ Attorney   &        0.04&        0.10&        0.06\sym{***}\\
                    &      (0.02)&      (0.11)&                     \\
 \textcolor{white}{...}Median Credit Score &      586.65&      688.71&      102.06\sym{***}\\
                    &     (50.98)&     (76.50)&                     \\
 \textcolor{white}{...}90+ DPD Debt Balances       &     3193.18&     1416.45&    -1776.73\sym{***}\\
                    &   (2676.72)&   (4253.49)&                     \\
\textbf{Panel B: Additional Neighborhood Characteristics} & & & \\ 
 \textcolor{white}{...}GINI Index &        0.46&        0.40&       -0.06\sym{***}\\
                    &      (0.05)&      (0.07)&                     \\

 \textcolor{white}{...}Unemployment Rate  &        0.12&        0.05&       -0.07\sym{***}\\
                    &      (0.05)&      (0.04)&                     \\
 \textcolor{white}{...}Divorce Rate&        0.13&        0.12&       -0.01\sym{***}\\
                    &      (0.03)&      (0.06)&                     \\
 \textcolor{white}{...}Fraction with Bachelors Degree&              0.16&        0.17&        0.00         \\
                    &      (0.10)&      (0.13)&                     \\
\textcolor{white}{...}Home Ownership Rate &        0.47&        0.76&        0.29\sym{***}\\
                    &      (0.19)&      (0.14)&                     \\
\textcolor{white}{...}Banks (5 miles)     &       85.44&       11.88&      -73.56\sym{***}\\
                    &     (40.79)&     (30.95)&                     \\
 \textcolor{white}{...}Payday Lenders (5 miles)&       29.98&        3.23&      -26.75\sym{***}\\
                    &      (9.86)&      (7.76)&                     \\
 \textcolor{white}{...}Zillow: Single Family House (in 000s) &       90.15&      122.26&       32.11\sym{***}\\
                    &     (54.29)&     (68.87)&                     \\
 \textcolor{white}{...}HMDA: Share Rejected, Black - White&        0.19&        0.15&       -0.04\sym{***}\\
                    &      (0.11)&      (0.31)&                     \\
 \textcolor{white}{...}Mean Household Income from IRS (in 000s) &       28.67&       41.01&       12.34\sym{***}\\
                    &     (10.00)&     (24.25)&                     \\

\hline
Zip Codes       &         258&        9530&           \\
Population &    17697 &     5808 &   \\
\hline\hline
\end{tabular}
   \begin{tablenotes}
     \scriptsize
    \item Notes:  This table presents summary statistics for the entire Missouri neighborhood level data from 2004-2013. Column 1 displays the sample means and standard deviations for neighborhoods in which at least 50\% of the population is black and column 2 displays sample means and standard deviations for neighborhoods in which less than 50\% is black.  The third column reports the difference in means across the two samples. \sym{*} \(p<0.10\), \sym{**} \(p<0.05\), \sym{***} \(p<0.01\)
   \end{tablenotes}
\end{threeparttable}
\end{table}
\begin{table}[htbp] \centering
\begin{threeparttable}
\footnotesize
\def\sym#1{\ifmmode^{#1}\else\(^{#1}\)\fi}
\caption{Judgments and Debt Portfolios: Entire Sample\label{tab:debt_composition_off_common}}
\begin{tabular}{l*{5}{c}}
\hline\hline
                    &\multicolumn{1}{c}{(1)}&\multicolumn{1}{c}{(2)}&\multicolumn{1}{c}{(3)}&\multicolumn{1}{c}{(4)}&\multicolumn{1}{c}{(5)}\\
                       &\multicolumn{5}{c}{Judgment Rate}\\
\hline
& & & & & \\[\dimexpr-\normalbaselineskip+2pt]
Black Majority: ZIP &      0.6926\sym{***}&      0.7086\sym{***}&      0.7058\sym{***}&      0.6957\sym{***}&      0.6871\sym{***}\\
                    &    (0.1549)         &    (0.1599)         &    (0.1594)         &    (0.1558)         &    (0.1476)         \\
\hline
& & & & &  \\[\dimexpr-\normalbaselineskip+2pt]
Debt Levels         &           X         &                     &                     &                     &           X         \\
Monthly Payment and Utilization&                     &           X         &                     &                     &           X         \\
Debt Composition    &                     &                     &           X         &                     &           X         \\
Delinquency/Bankruptcy/Collections&                     &                     &                     &           X         &           X         \\
\hline
& & & & & \\[\dimexpr-\normalbaselineskip+2pt]
Wild Cluster Bootstrap p-value&       .0004         &       .0005         &       .0005         &       .0004         &       .0003         \\
Observations        &   7484        &   7484        &   7484        &   7484        &   7484        \\
$R^2$               &      0.7037         &      0.7021         &      0.7020         &      0.7038         &      0.7079         \\
\hline\hline
\end{tabular}
\begin{tablenotes}
\scriptsize
\item Notes:  This table presents results of a regression of the judgment rate on neighborhood racial composition and other neighborhood-level characteristics.  The sample includes the entire Missouri zip code sample.  The dependent variable is judgments per 100 individuals.  Baseline controls include average zip code-level income, the fraction of IRS filings under \$25,000, between \$25,000-50,000, \$50,000-75,000, \$75,000-100,000, and over \$100,000, credit score quintiles, median credit score, total delinquent debt balances, unemployment rate, median house value, the fraction of the population with a college education, the divorce rate, and population density.  Baseline controls, county fixed effects, and year fixed effects are included in all specifications, and all regressions are weighted by population. Robust standard errors clustered at the county-year level are in parentheses. Effective number of clusters: 36.0. Wild Cluster Bootstrap p-values are reported for our main parameter of interest. \sym{*} \(p<0.10\), \sym{**} \(p<0.05\), \sym{***} \(p<0.01\). 
\end{tablenotes}
\end{threeparttable}
\end{table}

\begin{sidewaystable}[htbp]\centering
\begin{threeparttable}
\footnotesize
\def\sym#1{\ifmmode^{#1}\else\(^{#1}\)\fi}
\caption{Attorney Representation and Judgment Type: Entire Sample\label{tab:judgment_type_off_common}}
\begin{tabular}{l*{9}{c}}
\hline\hline
                    &\multicolumn{1}{c}{(1)}&\multicolumn{1}{c}{(2)}&\multicolumn{1}{c}{(3)}&\multicolumn{1}{c}{(4)}&\multicolumn{1}{c}{(5)}&\multicolumn{1}{c}{(6)}&\multicolumn{1}{c}{(7)}&\multicolumn{1}{c}{(8)}&\multicolumn{1}{c}{(9)}\\
                    &\multicolumn{1}{c}{Attorney}&\multicolumn{1}{c}{Judgments}&\multicolumn{1}{c}{Judgments}&\multicolumn{1}{c}{Consent}&\multicolumn{1}{c}{Contested}&\multicolumn{1}{c}{Default}&\multicolumn{1}{c}{Dismissed}&\multicolumn{1}{c}{Settle}&\multicolumn{1}{c}{Judgments}\\
\hline
&&&&& & & & \\[\dimexpr-\normalbaselineskip+2pt]
Black Majority: ZIP &      -0.016\sym{***}&       0.685\sym{***}&       0.706\sym{***}&       0.004         &       0.001         &       0.014\sym{***}&       0.010         &      -0.022\sym{***} &       0.752\sym{***}\\
                    &     (0.003)         &     (0.155)         &     (0.160)         &     (0.005)         &     (0.004)         &     (0.005)         &     (0.007)         &     (0.006)    & (0.162)     \\
\hline
&&&&& & & & &\\[\dimexpr-\normalbaselineskip+2pt]
Attorney Representation & & X & X&X&X&X&X&X&X \\
Lagged Case Outcomes & & & & & & & & & X \\ \hline 
&&&&& & & & S \\[\dimexpr-\normalbaselineskip+2pt]
Wild Cluster Bootstrap p-value&           0         &       .0004         &       .0004         &       .4475         &       .8498         &       .0096         &       .1681         &       .0036    & 0.0008     \\
Observations        &    7484       &    7484       &    7484       &    7484       &    7484       &    7484       &    7484       &    7484    & 6701   \\
$R^2$               &       0.440         &       0.715         &       0.702         &       0.479         &       0.407         &       0.389         &       0.654         &       0.643     & 0.732    \\
\hline\hline
\end{tabular}
\begin{tablenotes}
\scriptsize
\item Notes:  This table explores the extent to which attorney representation or previous case outcomes can explain the racial gap in judgments.  The sample includes the entire Missouri zip code level sample. The outcome variable in Column (1) is the share of debt collection court cases where an attorney represented the defendant.  The outcome variable in columns (2) and (8) are judgments per 100 people.  The outcome variables in Columns (3)-(7) are the share of cases resulting in a consent judgment, a contested judgment, a default judgment, the case being dismissed, and the case being settled, respectively.  All regressions are weighted by population. Baseline controls (average zip code-level income, the fraction of IRS filings under \$25,000, between \$25,000-50,000, \$50,000-75,000, \$75,000-100,000, and over \$100,000, credit score quintiles, median credit score, total delinquent debt balances, unemployment rate, median house value, the fraction of the population with a college education, the divorce rate, and population density), county fixed effects, and year fixed effects are included in all specifications. Aside from Column (1), all specifications control for the share of cases with attorney representation. Column (8) controls for the share of default judgments. Robust standard errors clustered at the county-year level are in parentheses. Effective number of clusters: 36.0. Wild Cluster Bootstrap p-values are reported for our main parameter of interest. \sym{*} \(p<0.10\), \sym{**} \(p<0.05\), \sym{***} \(p<0.01\). 
\end{tablenotes}
\end{threeparttable}
\end{sidewaystable}

\begin{table}[htbp] \centering
\begin{threeparttable}
\footnotesize
\def\sym#1{\ifmmode^{#1}\else\(^{#1}\)\fi}
\caption{Judgments and Other Demographic Groups\label{tab:race_other}}
\begin{tabular}{l*{6}{c}}
\hline\hline
                    &\multicolumn{1}{c}{(1)}&\multicolumn{1}{c}{(2)}&\multicolumn{1}{c}{(3)}&\multicolumn{1}{c}{(4)}&\multicolumn{1}{c}{(5)}&\multicolumn{1}{c}{(6)}\\
                       &\multicolumn{6}{c}{Judgment Rate}\\
\hline
& & & & & & \\[\dimexpr-\normalbaselineskip+2pt]
Share Black: ZIP    &      2.2881\sym{***}&      1.5574\sym{***}&      1.9195\sym{***}&      1.4544\sym{***}&      1.4865\sym{***}&      1.6260\sym{***}\\
                    &    (0.2748)         &    (0.3184)         &    (0.2505)         &    (0.2955)         &    (0.2777)         &    (0.0610)         \\
& & & & & & \\[\dimexpr-\normalbaselineskip+2pt]
Share Asian: ZIP    &     -5.6745\sym{***}&     -3.3050\sym{***}&     -4.8311\sym{***}&     -3.1980\sym{***}&     -1.6851\sym{**} &     -3.6100\sym{***}\\
                    &    (0.9938)         &    (0.9074)         &    (0.9953)         &    (0.8989)         &    (0.7889)         &    (0.4954)         \\
& & & & & & \\[\dimexpr-\normalbaselineskip+2pt]
Share Hispanic: ZIP &      1.0901\sym{***}&     -0.3160\sym{***}&      0.7415\sym{***}&     -0.3814\sym{***}&      0.5452\sym{***}&     -0.3274\sym{*}  \\
                    &    (0.1345)         &    (0.1217)         &    (0.1357)         &    (0.1297)         &    (0.1421)         &    (0.1820)         \\
\hline
& & & & & & \\[\dimexpr-\normalbaselineskip+2pt]
Baseline Controls   &                     &                     &                     &                     &           X         &                     \\
Income     &                     &           X         &                     &           X         &           X         &                     \\
Credit Score  &                     &                     &           X         &           X         &           X         &                     \\
Lagged Baseline Controls&                     &                     &                     &                     &                     &           X         \\ \hline
& & & & & & \\[\dimexpr-\normalbaselineskip+2pt]
Wild Cluster Bootstrap p$_{\text{Black}}$&           0         &           0         &           0         &           0         &           0         &           0         \\
Wild Cluster Bootstrap p$_{\text{Hispanic}}$&           0         &       .0137         &       .0001         &        .008         &       .0003         &       .1084         \\
Wild Cluster Bootstrap p$_{\text{Asian}}$&           0         &       .0031         &       .0002         &       .0026         &       .0552         &           0         \\
Observations        &   7365        &   7365        &   7019        &   7019        &   7019        &   6105        \\
$R^2$               &      0.6496         &      0.6796         &      0.6618         &      0.6841         &      0.6973         &      0.6952         \\
\hline\hline
\end{tabular}
\begin{tablenotes}
\scriptsize
\item Notes:  This table presents results of a regression of the judgment rate on neighborhood racial composition and other neighborhood-level characteristics.  The sample includes Missouri zip codes in the common support sample.  The dependent variable is judgments per 100 individuals.  Baseline controls include average zip code-level income, the fraction of IRS filings under \$25,000, between \$25,000-50,000, \$50,000-75,000, \$75,000-100,000, and over \$100,000, credit score quintiles, median credit score, total delinquent debt balances, unemployment rate, median house value, the fraction of the population with a college education, the divorce rate, and population density.  Baseline controls, county fixed effects, and year fixed effects are included in all specifications, and all regressions are weighted by population. Robust standard errors clustered at the county-year level are in parentheses. Effective number of clusters: 36.0. Wild Cluster Bootstrap p-values are reported for our main parameter of interest. \sym{*} \(p<0.10\), \sym{**} \(p<0.05\), \sym{***} \(p<0.01\). 
\end{tablenotes}
\end{threeparttable}
\end{table}
\begin{table}[htbp]\centering
\begin{threeparttable}
\footnotesize
\caption{Judgments and Double Machine Learning\label{tab:dml}}
\begin{tabular}{l*{5}{c}} \hline \hline
 & R2: Y Model & R2: T Model & Estimates & T-values \\ \hline 
 & & &  & \\[\dimexpr-\normalbaselineskip+2pt]
T: Majority Black & 0.5121 & 0.9877 & 1.020 & 1.824 \\
 & [0.0069] & [0.0022] & [0.2682] & [0.4028] \\ \hline \hline
% & & &  & \\[\dimexpr-\normalbaselineskip+2pt]
%T: Continuous & 0.5121 &  0.9904 & 3.909 & 6.8267 \\
% & [0.0069] & [0.0015] & [0.4592] & [1.3375] \\ \hline \hline 
\end{tabular}
\begin{tablenotes}
\scriptsize
\item Notes: We use five-fold cross-validation in the first stage. Features used correspond to Column (5) of Table \ref{tab:creditworthiness}. For the classification tasks, we use Gradient Boosted Trees, while for the regression tasks, we use Random Forest.  We repeat the estimation with different seeds 1,000 times with distinct train-test splits and the statistics reported are the averages obtained from this exercise. Standard deviations are in brackets.
\end{tablenotes}
\end{threeparttable}
\end{table}
\clearpage
